# Supplementary material for: Noise limits on two-photon interferometric sensing
Source: arXiv:2106.13671 ancillary file (2021-08-25)
Supplement: Supplementary file 1 [file equations_full.pdf]

All functions take as input the four variables:

$\delta$  - the delay

$\alpha$  - the visibility

$\sigma$  - the spectral width

$\omega_p$  - the pump frequency

The fixed shift probabilities take additional variables for the shifts. For mode-correlated noise, these are the two variables:

$\epsilon$  - the frequency-dependent shift

$\theta$  - the frequency-independent shift

For mode-uncorrelated noise, there are four shift variables:

$\epsilon_1$  - the frequency-dependent shift for the c mode

$\epsilon_2$  - the frequency-dependent shift for the d mode

$\theta_1$  - the frequency-independent shift for the c mode

$\theta_2$  - the frequency-independent shift for the d mode

The noisy probabilities and Fisher information instead take the additional variables:

$\eta\epsilon$  - the degree of frequency-dependent noise

$\eta\theta$  - the degree of frequency-independent noise

Variables are generally included in function even if the specific expression had no dependence on certain variables (such as HOM having no  $\omega_p$  dependence, or the lack of visibility dependence in certain configurations)

$P_1, P_2, P_c$  are the probabilities for detection at detector 1, detector 2, or a coincidence at both detectors respectively

$F$  is the Fisher information

# HOM

---

## Frequency-entangled photons

### Fixed shift

$$P_{1\text{HOM}}[\delta_-, \alpha_-, \sigma_-, \omega_{p-}, \epsilon_-, \theta_-] := \frac{1}{4} \left( 1 + e^{-2(\delta-\epsilon)^2 \sigma^2} \alpha \right)$$

$$P_{2\text{HOM}}[\delta_-, \alpha_-, \sigma_-, \omega_{p-}, \epsilon_-, \theta_-] := \frac{1}{4} \left( 1 + e^{-2(\delta-\epsilon)^2 \sigma^2} \alpha \right)$$

$$P_{c\text{HOM}}[\delta_-, \alpha_-, \sigma_-, \omega_{p-}, \epsilon_-, \theta_-] := \frac{1}{2} \left( 1 - e^{-2(\delta-\epsilon)^2 \sigma^2} \alpha \right)$$

## Noisy

$$\ln[*]:= \text{P1HOM}\eta[\delta\_ , \alpha\_ , \sigma\_ , \omega\text{p}\_ , \eta\epsilon\_ , \eta\theta\_ ] := \frac{1}{4} \left( 1 + \frac{e^{-\frac{2\delta^2\sigma^2}{1+4\eta\epsilon^2\sigma^2}} \alpha}{\sqrt{1+4\eta\epsilon^2\sigma^2}} \right)$$

$$\text{P2HOM}\eta[\delta\_ , \alpha\_ , \sigma\_ , \omega\text{p}\_ , \eta\epsilon\_ , \eta\theta\_ ] := \frac{1}{4} \left( 1 + \frac{e^{-\frac{2\delta^2\sigma^2}{1+4\eta\epsilon^2\sigma^2}} \alpha}{\sqrt{1+4\eta\epsilon^2\sigma^2}} \right)$$

$$\text{PcHOM}\eta[\delta\_ , \alpha\_ , \sigma\_ , \omega\text{p}\_ , \eta\epsilon\_ , \eta\theta\_ ] := \frac{1}{2} \left( 1 - \frac{e^{-\frac{2\delta^2\sigma^2}{1+4\eta\epsilon^2\sigma^2}} \alpha}{\sqrt{1+4\eta\epsilon^2\sigma^2}} \right)$$

$$\ln[*]:= \text{FHOM}\eta[\delta\_ , \alpha\_ , \sigma\_ , \omega\text{p}\_ , \eta\epsilon\_ , \eta\theta\_ ] := \frac{16\alpha^2\delta^2\sigma^4}{(1+4\eta\epsilon^2\sigma^2)^2 \left( -\alpha^2 + e^{\frac{4\delta^2\sigma^2}{1+4\eta\epsilon^2\sigma^2}} (1+4\eta\epsilon^2\sigma^2) \right)}$$

## Frequency-independent photons

### Fixed shift

$$\text{P1HOMind}[\delta\_ , \alpha\_ , \sigma\_ , \omega\text{p}\_ , \epsilon\_ , \theta\_ ] := \frac{1}{4} \left( 1 + e^{-(\delta-\epsilon)^2\sigma^2} \alpha \right)$$

$$\text{P2HOMind}[\delta\_ , \alpha\_ , \sigma\_ , \omega\text{p}\_ , \epsilon\_ , \theta\_ ] := \frac{1}{4} \left( 1 + e^{-(\delta-\epsilon)^2\sigma^2} \alpha \right)$$

$$\text{PcHOMind}[\delta\_ , \alpha\_ , \sigma\_ , \omega\text{p}\_ , \epsilon\_ , \theta\_ ] := \frac{1}{2} - \frac{1}{2} e^{-(\delta-\epsilon)^2\sigma^2} \alpha$$

## Noisy

$$\ln[*]:= \text{P1HOMind}\eta[\delta\_ , \alpha\_ , \sigma\_ , \omega\text{p}\_ , \eta\epsilon\_ , \eta\theta\_ ] := \frac{1}{4} \left( 1 + \frac{e^{-\frac{\delta^2\sigma^2}{1+2\eta\epsilon^2\sigma^2}} \alpha}{\sqrt{1+2\eta\epsilon^2\sigma^2}} \right)$$

$$\text{P2HOMind}\eta[\delta\_ , \alpha\_ , \sigma\_ , \omega\text{p}\_ , \eta\epsilon\_ , \eta\theta\_ ] := \frac{1}{4} \left( 1 + \frac{e^{-\frac{\delta^2\sigma^2}{1+2\eta\epsilon^2\sigma^2}} \alpha}{\sqrt{1+2\eta\epsilon^2\sigma^2}} \right)$$

$$\text{PcHOMind}\eta[\delta\_ , \alpha\_ , \sigma\_ , \omega\text{p}\_ , \eta\epsilon\_ , \eta\theta\_ ] := \frac{1}{2} \left( 1 - \frac{e^{-\frac{\delta^2\sigma^2}{1+2\eta\epsilon^2\sigma^2}} \alpha}{\sqrt{1+2\eta\epsilon^2\sigma^2}} \right)$$

$$\ln[*]:= \text{FHOMind}\eta[\delta\_ , \alpha\_ , \sigma\_ , \omega\text{p}\_ , \eta\epsilon\_ , \eta\theta\_ ] := \frac{4\alpha^2\delta^2\sigma^4}{(1+2\eta\epsilon^2\sigma^2)^2 \left( -\alpha^2 + e^{\frac{2\delta^2\sigma^2}{1+2\eta\epsilon^2\sigma^2}} (1+2\eta\epsilon^2\sigma^2) \right)}$$

# MZ1

## Fixed shift

$$P1sing[\delta_-, \alpha_-, \sigma_-, \omega p_-, \epsilon_-, \theta_-] := \frac{1}{2} \left( 1 - e^{-\frac{1}{2}(\delta-\epsilon)^2 \sigma^2} \cos \left[ \theta - \frac{(\delta-\epsilon) \omega p_-}{2} \right] \right)$$

$$P2sing[\delta_-, \alpha_-, \sigma_-, \omega p_-, \epsilon_-, \theta_-] := \frac{1}{2} \left( 1 + e^{-\frac{1}{2}(\delta-\epsilon)^2 \sigma^2} \cos \left[ \theta - \frac{(\delta-\epsilon) \omega p_-}{2} \right] \right)$$

## Noisy

$$In[*]:= P1sing\eta[\delta_-, \alpha_-, \sigma_-, \omega p_-, \eta\epsilon_-, \eta\theta_-] := \frac{1}{2} \left( 1 - \frac{e^{-\frac{4(\eta\theta^2 + (\delta^2 + \eta\epsilon^2 \eta\theta^2) \sigma^2) + \eta\epsilon^2 \omega p_-^2}{8+8\eta\epsilon^2 \sigma^2}} \cos \left[ \frac{\delta \omega p_-}{2+2\eta\epsilon^2 \sigma^2} \right]}{\sqrt{1 + \eta\epsilon^2 \sigma^2}} \right)$$

$$In[*]:= P2sing\eta[\delta_-, \alpha_-, \sigma_-, \omega p_-, \eta\epsilon_-, \eta\theta_-] := \frac{1}{2} \left( 1 + \frac{e^{-\frac{4\delta^2 \sigma^2 + 4\eta\theta^2 (1+\eta\epsilon^2 \sigma^2) + \eta\epsilon^2 \omega p_-^2}{8+8\eta\epsilon^2 \sigma^2}} \cos \left[ \frac{\delta \omega p_-}{2+2\eta\epsilon^2 \sigma^2} \right]}{\sqrt{1 + \eta\epsilon^2 \sigma^2}} \right)$$

$$In[*]:= Fsing\eta[\delta_-, \alpha_-, \sigma_-, \omega p_-, \eta\epsilon_-, \eta\theta_-] := \frac{\left( 2 \delta \sigma^2 \cos \left[ \frac{\delta \omega p_-}{2+2\eta\epsilon^2 \sigma^2} \right] + \omega p_- \sin \left[ \frac{\delta \omega p_-}{2+2\eta\epsilon^2 \sigma^2} \right] \right)^2}{4 (1 + \eta\epsilon^2 \sigma^2)^2 \left( e^{-\frac{4(\eta\theta^2 + (\delta^2 + \eta\epsilon^2 \eta\theta^2) \sigma^2) + \eta\epsilon^2 \omega p_-^2}{4+4\eta\epsilon^2 \sigma^2}} (1 + \eta\epsilon^2 \sigma^2) - \cos \left[ \frac{\delta \omega p_-}{2+2\eta\epsilon^2 \sigma^2} \right]^2 \right)}$$

# MZ2s

## Mode-correlated noise

## Frequency-entangled photons

### Fixed shift

$$P1s[\delta_-, \alpha_-, \sigma_-, \omega p_-, \epsilon_-, \theta_-] := \frac{1}{8} \left( 2 + e^{-2(\delta-\epsilon)^2 \sigma^2} + \cos[2\theta - \delta \omega p_- + \epsilon \omega p_-] - 4 e^{-\frac{1}{2}(\delta-\epsilon)^2 \sigma^2} \cos \left[ \theta + \frac{1}{2}(-\delta + \epsilon) \omega p_- \right] \right)$$

$$P2s[\delta_-, \alpha_-, \sigma_-, \omega p_-, \epsilon_-, \theta_-] := \frac{1}{8} \left( 2 + e^{-2(\delta-\epsilon)^2 \sigma^2} + \cos[2\theta - \delta \omega p_- + \epsilon \omega p_-] + 4 e^{-\frac{1}{2}(\delta-\epsilon)^2 \sigma^2} \cos \left[ \theta + \frac{1}{2}(-\delta + \epsilon) \omega p_- \right] \right)$$

$$Pcs[\delta_-, \alpha_-, \sigma_-, \omega p_-, \epsilon_-, \theta_-] := \frac{1}{4} \left( 2 - e^{-2(\delta-\epsilon)^2 \sigma^2} - \cos[2\theta + (-\delta + \epsilon) \omega p_-] \right)$$

## Noisy

$$\ln[*]:= \text{P1s}\eta[\delta\_ , \alpha\_ , \sigma\_ , \omega\rho\_ , \eta\epsilon\_ , \eta\theta\_ ] :=$$

$$\frac{1}{8} \left( 2 + \frac{e^{-\frac{2\delta^2\sigma^2}{1+4\eta\epsilon^2\sigma^2}}}{\sqrt{1+4\eta\epsilon^2\sigma^2}} + e^{-2\eta\theta^2 - \frac{\eta\epsilon^2\omega\rho^2}{2}} \text{Cos}[\delta\omega\rho] - \frac{4e^{-\frac{4\delta^2\sigma^2+4\eta\theta^2(1+\eta\epsilon^2\sigma^2)+\eta\epsilon^2\omega\rho^2}{8+8\eta\epsilon^2\sigma^2}} \text{Cos}\left[\frac{\delta\omega\rho}{2+2\eta\epsilon^2\sigma^2}\right]}{\sqrt{1+\eta\epsilon^2\sigma^2}} \right)$$

$$\ln[*]:= \text{P2s}\eta[\delta\_ , \alpha\_ , \sigma\_ , \omega\rho\_ , \eta\epsilon\_ , \eta\theta\_ ] :=$$

$$\frac{1}{8} \left( 2 + \frac{e^{-\frac{2\delta^2\sigma^2}{1+4\eta\epsilon^2\sigma^2}}}{\sqrt{1+4\eta\epsilon^2\sigma^2}} + e^{-2\eta\theta^2 - \frac{\eta\epsilon^2\omega\rho^2}{2}} \text{Cos}[\delta\omega\rho] + \frac{4e^{-\frac{4\delta^2\sigma^2+4\eta\theta^2(1+\eta\epsilon^2\sigma^2)+\eta\epsilon^2\omega\rho^2}{8+8\eta\epsilon^2\sigma^2}} \text{Cos}\left[\frac{\delta\omega\rho}{2+2\eta\epsilon^2\sigma^2}\right]}{\sqrt{1+\eta\epsilon^2\sigma^2}} \right)$$

$$\ln[*]:= \text{Pcs}\eta[\delta\_ , \alpha\_ , \sigma\_ , \omega\rho\_ , \eta\epsilon\_ , \eta\theta\_ ] := \frac{1}{4} \left( 2 - \frac{e^{-\frac{2\delta^2\sigma^2}{1+4\eta\epsilon^2\sigma^2}}}{\sqrt{1+4\eta\epsilon^2\sigma^2}} - e^{-2\eta\theta^2 - \frac{\eta\epsilon^2\omega\rho^2}{2}} \text{Cos}[\delta\omega\rho] \right)$$

$$\ln[*]:= \text{Fs}\eta[\delta\_ , \alpha\_ , \sigma\_ , \omega\rho\_ , \eta\epsilon\_ , \eta\theta\_ ] := \frac{\left( \frac{4e^{-\frac{2\delta^2\sigma^2}{1+4\eta\epsilon^2\sigma^2}}\delta\sigma^2}{(1+4\eta\epsilon^2\sigma^2)^{3/2}} + e^{-2\eta\theta^2 - \frac{\eta\epsilon^2\omega\rho^2}{2}}\omega\rho \text{Sin}[\delta\omega\rho] \right)^2}{4 \left( 2 - \frac{e^{-\frac{2\delta^2\sigma^2}{1+4\eta\epsilon^2\sigma^2}}}{\sqrt{1+4\eta\epsilon^2\sigma^2}} - e^{-2\eta\theta^2 - \frac{\eta\epsilon^2\omega\rho^2}{2}} \text{Cos}[\delta\omega\rho] \right)} +$$

$$\left( \frac{4e^{-\frac{2\delta^2\sigma^2}{1+4\eta\epsilon^2\sigma^2}}\delta\sigma^2}{(1+4\eta\epsilon^2\sigma^2)^{3/2}} - \frac{4e^{-\frac{4\delta^2\sigma^2+4\eta\theta^2(1+\eta\epsilon^2\sigma^2)+\eta\epsilon^2\omega\rho^2}{8+8\eta\epsilon^2\sigma^2}}\delta\sigma^2 \text{Cos}\left[\frac{\delta\omega\rho}{2+2\eta\epsilon^2\sigma^2}\right]}{(1+\eta\epsilon^2\sigma^2)^{3/2}} + \right.$$

$$\left. e^{-2\eta\theta^2 - \frac{\eta\epsilon^2\omega\rho^2}{2}}\omega\rho \text{Sin}[\delta\omega\rho] - \frac{2e^{-\frac{4\delta^2\sigma^2+4\eta\theta^2(1+\eta\epsilon^2\sigma^2)+\eta\epsilon^2\omega\rho^2}{8+8\eta\epsilon^2\sigma^2}}\omega\rho \text{Sin}\left[\frac{\delta\omega\rho}{2+2\eta\epsilon^2\sigma^2}\right]}{(1+\eta\epsilon^2\sigma^2)^{3/2}} \right)^2 /$$

$$\left( 8 \left( 2 + \frac{e^{-\frac{2\delta^2\sigma^2}{1+4\eta\epsilon^2\sigma^2}}}{\sqrt{1+4\eta\epsilon^2\sigma^2}} + e^{-2\eta\theta^2 - \frac{\eta\epsilon^2\omega\rho^2}{2}} \text{Cos}[\delta\omega\rho] - \frac{4e^{-\frac{4\delta^2\sigma^2+4\eta\theta^2(1+\eta\epsilon^2\sigma^2)+\eta\epsilon^2\omega\rho^2}{8+8\eta\epsilon^2\sigma^2}} \text{Cos}\left[\frac{\delta\omega\rho}{2+2\eta\epsilon^2\sigma^2}\right]}{\sqrt{1+\eta\epsilon^2\sigma^2}} \right) \right) +$$

$$\left( \frac{4e^{-\frac{2\delta^2\sigma^2}{1+4\eta\epsilon^2\sigma^2}}\delta\sigma^2}{(1+4\eta\epsilon^2\sigma^2)^{3/2}} + \frac{4e^{-\frac{4\delta^2\sigma^2+4\eta\theta^2(1+\eta\epsilon^2\sigma^2)+\eta\epsilon^2\omega\rho^2}{8+8\eta\epsilon^2\sigma^2}}\delta\sigma^2 \text{Cos}\left[\frac{\delta\omega\rho}{2+2\eta\epsilon^2\sigma^2}\right]}{(1+\eta\epsilon^2\sigma^2)^{3/2}} + \right.$$

$$\left. e^{-2\eta\theta^2 - \frac{\eta\epsilon^2\omega\rho^2}{2}}\omega\rho \text{Sin}[\delta\omega\rho] + \frac{2e^{-\frac{4\delta^2\sigma^2+4\eta\theta^2(1+\eta\epsilon^2\sigma^2)+\eta\epsilon^2\omega\rho^2}{8+8\eta\epsilon^2\sigma^2}}\omega\rho \text{Sin}\left[\frac{\delta\omega\rho}{2+2\eta\epsilon^2\sigma^2}\right]}{(1+\eta\epsilon^2\sigma^2)^{3/2}} \right)^2 /$$

$$\left( 8 \left( 2 + \frac{e^{-\frac{2\delta^2\sigma^2}{1+4\eta\epsilon^2\sigma^2}}}{\sqrt{1+4\eta\epsilon^2\sigma^2}} + e^{-2\eta\theta^2 - \frac{\eta\epsilon^2\omega\rho^2}{2}} \text{Cos}[\delta\omega\rho] + \frac{4e^{-\frac{4\delta^2\sigma^2+4\eta\theta^2(1+\eta\epsilon^2\sigma^2)+\eta\epsilon^2\omega\rho^2}{8+8\eta\epsilon^2\sigma^2}} \text{Cos}\left[\frac{\delta\omega\rho}{2+2\eta\epsilon^2\sigma^2}\right]}{\sqrt{1+\eta\epsilon^2\sigma^2}} \right) \right)$$

# Frequency-independent photons

## Fixed shift

$$\ln[*]:= \text{P1sind}[\delta\_ , \sigma\_ , \omega p\_ , \epsilon\_ , \theta\_ ] := \frac{1}{4} e^{-(\delta^2 + \epsilon^2) \sigma^2} \left( e^{\frac{1}{2} (\delta^2 + \epsilon^2) \sigma^2} - e^{\delta \epsilon \sigma^2} \cos \left[ \theta + \frac{1}{2} (-\delta + \epsilon) \omega p \right] \right)^2$$

$$\ln[*]:= \text{P2sind}[\delta\_ , \sigma\_ , \omega p\_ , \epsilon\_ , \theta\_ ] := \frac{1}{4} e^{-(\delta^2 + \epsilon^2) \sigma^2} \left( e^{\frac{1}{2} (\delta^2 + \epsilon^2) \sigma^2} + e^{\delta \epsilon \sigma^2} \cos \left[ \theta + \frac{1}{2} (-\delta + \epsilon) \omega p \right] \right)^2$$

$$\ln[*]:= \text{Pcsind}[\delta\_ , \sigma\_ , \omega p\_ , \epsilon\_ , \theta\_ ] := -\frac{1}{4} e^{-(\delta^2 + \epsilon^2) \sigma^2} \left( e^{2 \delta \epsilon \sigma^2} - 2 e^{(\delta^2 + \epsilon^2) \sigma^2} + e^{2 \delta \epsilon \sigma^2} \cos [2 \theta + (-\delta + \epsilon) \omega p] \right)$$

## Noisy

$$\ln[*]:= \text{P1sind}\eta[\delta\_ , \alpha\_ , \sigma\_ , \omega p\_ , \eta \epsilon\_ , \eta \theta\_ ] := \left( e^{-\frac{\delta^2 \sigma^2 (3+2 \eta \epsilon^2 \sigma^2) + \eta \theta^2 (4+8 \eta \epsilon^2 \sigma^2) + \eta \epsilon^2 \omega p^2}{2+4 \eta \epsilon^2 \sigma^2}} \left( e^{\frac{\eta \theta^2 (4+8 \eta \epsilon^2 \sigma^2) + \delta^2 (\sigma^2 + 2 \eta \epsilon^2 \sigma^4) + \eta \epsilon^2 \omega p^2}{2+4 \eta \epsilon^2 \sigma^2}} \sqrt{1 + \eta \epsilon^2 \sigma^2} \left( 1 + 2 e^{\frac{\delta^2 \sigma^2}{1+2 \eta \epsilon^2 \sigma^2}} \sqrt{1 + 2 \eta \epsilon^2 \sigma^2} \right) + e^{\frac{\delta^2 \sigma^2}{2}} \sqrt{1 + \eta \epsilon^2 \sigma^2} \cos \left[ \frac{\delta \omega p}{1 + 2 \eta \epsilon^2 \sigma^2} \right] - 4 e^{\frac{12 \eta \theta^2 (1+3 \eta \epsilon^2 \sigma^2 + 2 \eta \epsilon^4 \sigma^4) + 4 \delta^2 \sigma^2 (2+3 \eta \epsilon^2 \sigma^2 + 2 \eta \epsilon^4 \sigma^4) + \eta \epsilon^2 (3+2 \eta \epsilon^2 \sigma^2) \omega p^2}{8 (1+3 \eta \epsilon^2 \sigma^2 + 2 \eta \epsilon^4 \sigma^4)}} \sqrt{1 + 2 \eta \epsilon^2 \sigma^2} \cos \left[ \frac{\delta \omega p}{2 + 2 \eta \epsilon^2 \sigma^2} \right] \right) \right) / \left( 8 \sqrt{1 + \eta \epsilon^2 \sigma^2} \sqrt{1 + 2 \eta \epsilon^2 \sigma^2} \right)$$

$$\ln[*]:= \text{P2sind}\eta[\delta\_ , \alpha\_ , \sigma\_ , \omega p\_ , \eta \epsilon\_ , \eta \theta\_ ] := \left( e^{-\frac{\delta^2 \sigma^2 (3+2 \eta \epsilon^2 \sigma^2) + \eta \theta^2 (4+8 \eta \epsilon^2 \sigma^2) + \eta \epsilon^2 \omega p^2}{2+4 \eta \epsilon^2 \sigma^2}} \left( e^{\frac{\eta \theta^2 (4+8 \eta \epsilon^2 \sigma^2) + \delta^2 (\sigma^2 + 2 \eta \epsilon^2 \sigma^4) + \eta \epsilon^2 \omega p^2}{2+4 \eta \epsilon^2 \sigma^2}} \sqrt{1 + \eta \epsilon^2 \sigma^2} \left( 1 + 2 e^{\frac{\delta^2 \sigma^2}{1+2 \eta \epsilon^2 \sigma^2}} \sqrt{1 + 2 \eta \epsilon^2 \sigma^2} \right) + e^{\frac{\delta^2 \sigma^2}{2}} \sqrt{1 + \eta \epsilon^2 \sigma^2} \cos \left[ \frac{\delta \omega p}{1 + 2 \eta \epsilon^2 \sigma^2} \right] + 4 e^{\frac{12 \eta \theta^2 (1+3 \eta \epsilon^2 \sigma^2 + 2 \eta \epsilon^4 \sigma^4) + 4 \delta^2 \sigma^2 (2+3 \eta \epsilon^2 \sigma^2 + 2 \eta \epsilon^4 \sigma^4) + \eta \epsilon^2 (3+2 \eta \epsilon^2 \sigma^2) \omega p^2}{8 (1+3 \eta \epsilon^2 \sigma^2 + 2 \eta \epsilon^4 \sigma^4)}} \sqrt{1 + 2 \eta \epsilon^2 \sigma^2} \cos \left[ \frac{\delta \omega p}{2 + 2 \eta \epsilon^2 \sigma^2} \right] \right) \right) / \left( 8 \sqrt{1 + \eta \epsilon^2 \sigma^2} \sqrt{1 + 2 \eta \epsilon^2 \sigma^2} \right)$$

$$\ln[*]:= \text{Pcsind}\eta[\delta\_ , \alpha\_ , \sigma\_ , \omega p\_ , \eta \epsilon\_ , \eta \theta\_ ] := \frac{1}{4} \left( 2 - \frac{e^{-\frac{\delta^2 \sigma^2}{1+2 \eta \epsilon^2 \sigma^2}}}{\sqrt{1 + 2 \eta \epsilon^2 \sigma^2}} - \frac{e^{-\frac{2 \delta^2 \sigma^2 + \eta \theta^2 (4+8 \eta \epsilon^2 \sigma^2) + \eta \epsilon^2 \omega p^2}{2+4 \eta \epsilon^2 \sigma^2}} \cos \left[ \frac{\delta \omega p}{1+2 \eta \epsilon^2 \sigma^2} \right]}{\sqrt{1 + 2 \eta \epsilon^2 \sigma^2}} \right)$$

$$\ln[*]:= \text{Fsind}\eta[\delta\_ , \alpha\_ , \sigma\_ , \omega p\_ , \eta \epsilon\_ , \eta \theta\_ ] := \frac{\left( \frac{2 e^{-\frac{\delta^2 \sigma^2}{1+2 \eta \epsilon^2 \sigma^2}} \delta \sigma^2}{(1+2 \eta \epsilon^2 \sigma^2)^{3/2}} + \frac{4 e^{-\frac{2 \delta^2 \sigma^2 + \eta \theta^2 (4+8 \eta \epsilon^2 \sigma^2) + \eta \epsilon^2 \omega p^2}{2+4 \eta \epsilon^2 \sigma^2}} \delta \sigma^2 \cos \left[ \frac{\delta \omega p}{1+2 \eta \epsilon^2 \sigma^2} \right]}{\sqrt{1+2 \eta \epsilon^2 \sigma^2} (2+4 \eta \epsilon^2 \sigma^2)} + \frac{e^{-\frac{2 \delta^2 \sigma^2 + \eta \theta^2 (4+8 \eta \epsilon^2 \sigma^2) + \eta \epsilon^2 \omega p^2}{2+4 \eta \epsilon^2 \sigma^2}} \omega p \sin \left[ \frac{\delta \omega p}{1+2 \eta \epsilon^2 \sigma^2} \right]}{(1+2 \eta \epsilon^2 \sigma^2)^{3/2}} \right)^2}{4 \left( 2 - \frac{e^{-\frac{\delta^2 \sigma^2}{1+2 \eta \epsilon^2 \sigma^2}}}{\sqrt{1+2 \eta \epsilon^2 \sigma^2}} - \frac{e^{-\frac{2 \delta^2 \sigma^2 + \eta \theta^2 (4+8 \eta \epsilon^2 \sigma^2) + \eta \epsilon^2 \omega p^2}{2+4 \eta \epsilon^2 \sigma^2}} \cos \left[ \frac{\delta \omega p}{1+2 \eta \epsilon^2 \sigma^2} \right]}{\sqrt{1+2 \eta \epsilon^2 \sigma^2}} \right)} + \left( 8 e^{\frac{\delta^2 \sigma^2 (3+2 \eta \epsilon^2 \sigma^2) + \eta \theta^2 (4+8 \eta \epsilon^2 \sigma^2) + \eta \epsilon^2 \omega p^2}{2+4 \eta \epsilon^2 \sigma^2}} \sqrt{1 + \eta \epsilon^2 \sigma^2} \sqrt{1 + 2 \eta \epsilon^2 \sigma^2} \right)$$



$$\begin{aligned}
& \sqrt{1 + \eta\epsilon^2 \sigma^2} \cos\left[\frac{\delta \omega p}{1 + 2 \eta\epsilon^2 \sigma^2}\right] - 4 e^{\frac{12 \eta\theta^2 (1+3 \eta\epsilon^2 \sigma^2 + 2 \eta\epsilon^4 \sigma^4) + 4 \delta^2 \sigma^2 (2+3 \eta\epsilon^2 \sigma^2 + 2 \eta\epsilon^4 \sigma^4) + \eta\epsilon^2 (3+2 \eta\epsilon^2 \sigma^2) \omega p^2}{8 (1+3 \eta\epsilon^2 \sigma^2 + 2 \eta\epsilon^4 \sigma^4)}} \\
& \sqrt{1 + 2 \eta\epsilon^2 \sigma^2} \cos\left[\frac{\delta \omega p}{2 + 2 \eta\epsilon^2 \sigma^2}\right] + \frac{1}{8 \sqrt{1 + \eta\epsilon^2 \sigma^2} \sqrt{1 + 2 \eta\epsilon^2 \sigma^2}} \\
& e^{-\frac{\delta^2 \sigma^2 (3+2 \eta\epsilon^2 \sigma^2) + \eta\theta^2 (4+8 \eta\epsilon^2 \sigma^2) + \eta\epsilon^2 \omega p^2}{2+4 \eta\epsilon^2 \sigma^2}} \left( \frac{4 e^{\frac{\delta^2 \sigma^2}{1+2 \eta\epsilon^2 \sigma^2} + \frac{\eta\theta^2 (4+8 \eta\epsilon^2 \sigma^2) + \delta^2 (\sigma^2 + 2 \eta\epsilon^2 \sigma^4) + \eta\epsilon^2 \omega p^2}{2+4 \eta\epsilon^2 \sigma^2}} \delta \sigma^2 \sqrt{1 + \eta\epsilon^2 \sigma^2}}{\sqrt{1 + 2 \eta\epsilon^2 \sigma^2}} + \right. \\
& \frac{1}{2 + 4 \eta\epsilon^2 \sigma^2} 2 e^{\frac{\eta\theta^2 (4+8 \eta\epsilon^2 \sigma^2) + \delta^2 (\sigma^2 + 2 \eta\epsilon^2 \sigma^4) + \eta\epsilon^2 \omega p^2}{2+4 \eta\epsilon^2 \sigma^2}} \delta \sqrt{1 + \eta\epsilon^2 \sigma^2} (\sigma^2 + 2 \eta\epsilon^2 \sigma^4) \\
& \left. \left( 1 + 2 e^{\frac{\delta^2 \sigma^2}{1+2 \eta\epsilon^2 \sigma^2}} \sqrt{1 + 2 \eta\epsilon^2 \sigma^2} \right) + e^{\frac{\delta^2 \sigma^2}{2}} \delta \sigma^2 \sqrt{1 + \eta\epsilon^2 \sigma^2} \cos\left[\frac{\delta \omega p}{1 + 2 \eta\epsilon^2 \sigma^2}\right] - \right. \\
& \left. \left( 4 e^{\frac{12 \eta\theta^2 (1+3 \eta\epsilon^2 \sigma^2 + 2 \eta\epsilon^4 \sigma^4) + 4 \delta^2 \sigma^2 (2+3 \eta\epsilon^2 \sigma^2 + 2 \eta\epsilon^4 \sigma^4) + \eta\epsilon^2 (3+2 \eta\epsilon^2 \sigma^2) \omega p^2}{8 (1+3 \eta\epsilon^2 \sigma^2 + 2 \eta\epsilon^4 \sigma^4)}} \delta \sigma^2 \sqrt{1 + 2 \eta\epsilon^2 \sigma^2} \right. \right. \\
& \left. \left. (2 + 3 \eta\epsilon^2 \sigma^2 + 2 \eta\epsilon^4 \sigma^4) \cos\left[\frac{\delta \omega p}{2 + 2 \eta\epsilon^2 \sigma^2}\right] \right) / \right. \\
& \left. (1 + 3 \eta\epsilon^2 \sigma^2 + 2 \eta\epsilon^4 \sigma^4) - \frac{e^{\frac{\delta^2 \sigma^2}{2}} \sqrt{1 + \eta\epsilon^2 \sigma^2} \omega p \sin\left[\frac{\delta \omega p}{1+2 \eta\epsilon^2 \sigma^2}\right]}{1 + 2 \eta\epsilon^2 \sigma^2} + \right. \\
& \left. \left. \frac{4 e^{\frac{12 \eta\theta^2 (1+3 \eta\epsilon^2 \sigma^2 + 2 \eta\epsilon^4 \sigma^4) + 4 \delta^2 \sigma^2 (2+3 \eta\epsilon^2 \sigma^2 + 2 \eta\epsilon^4 \sigma^4) + \eta\epsilon^2 (3+2 \eta\epsilon^2 \sigma^2) \omega p^2}{8 (1+3 \eta\epsilon^2 \sigma^2 + 2 \eta\epsilon^4 \sigma^4)}} \sqrt{1 + 2 \eta\epsilon^2 \sigma^2} \omega p \sin\left[\frac{\delta \omega p}{2+2 \eta\epsilon^2 \sigma^2}\right]}{2 + 2 \eta\epsilon^2 \sigma^2} \right) \right) \right) \\
& / \left( e^{\frac{\eta\theta^2 (4+8 \eta\epsilon^2 \sigma^2) + \delta^2 (\sigma^2 + 2 \eta\epsilon^2 \sigma^4) + \eta\epsilon^2 \omega p^2}{2+4 \eta\epsilon^2 \sigma^2}} \sqrt{1 + \eta\epsilon^2 \sigma^2} \left( 1 + 2 e^{\frac{\delta^2 \sigma^2}{1+2 \eta\epsilon^2 \sigma^2}} \sqrt{1 + 2 \eta\epsilon^2 \sigma^2} \right) + \right. \\
& e^{\frac{\delta^2 \sigma^2}{2}} \sqrt{1 + \eta\epsilon^2 \sigma^2} \cos\left[\frac{\delta \omega p}{1 + 2 \eta\epsilon^2 \sigma^2}\right] - \\
& \left. 4 e^{\frac{12 \eta\theta^2 (1+3 \eta\epsilon^2 \sigma^2 + 2 \eta\epsilon^4 \sigma^4) + 4 \delta^2 \sigma^2 (2+3 \eta\epsilon^2 \sigma^2 + 2 \eta\epsilon^4 \sigma^4) + \eta\epsilon^2 (3+2 \eta\epsilon^2 \sigma^2) \omega p^2}{8 (1+3 \eta\epsilon^2 \sigma^2 + 2 \eta\epsilon^4 \sigma^4)}} \sqrt{1 + 2 \eta\epsilon^2 \sigma^2} \cos\left[\frac{\delta \omega p}{2 + 2 \eta\epsilon^2 \sigma^2}\right] \right)
\end{aligned}$$

## Mode-uncorrelated noise

### Frequency-entangled photons

Fixed shift

$$\begin{aligned}
\ln[*]:= \text{P1s}\mu[\delta\_ , \alpha\_ , \sigma\_ , \omega p\_ , \epsilon 1\_ , \epsilon 2\_ , \theta 1\_ , \theta 2\_ ] &:= \frac{1}{8(1+\alpha)} e^{-\frac{1}{2}(4\delta^2+4\epsilon 1^2+2\epsilon 1\epsilon 2+\epsilon 2^2)\sigma^2} \\
&\left( 2e^{\frac{1}{2}(4\delta^2+4\epsilon 1^2+2\epsilon 1\epsilon 2+\epsilon 2^2)\sigma^2} + 2e^{\frac{1}{2}(8\delta\epsilon 1+2\epsilon 1\epsilon 2+\epsilon 2^2)\sigma^2} \alpha + 2e^{\frac{1}{2}(4\delta^2+4\epsilon 1^2+2\epsilon 1\epsilon 2+\epsilon 2^2)\sigma^2} \alpha - \right. \\
&2e^{\frac{1}{2}(3\delta^2+2\delta\epsilon 1+3\epsilon 1^2+2\epsilon 1\epsilon 2+\epsilon 2^2)\sigma^2} (1+3\alpha) \text{Cos}\left[\theta 1 + \frac{1}{2}(-\delta + \epsilon 1)\omega p\right] + \\
&2e^{\frac{1}{2}(4\delta^2+4\epsilon 1^2+2\epsilon 1\epsilon 2+\epsilon 2^2)\sigma^2} \alpha \text{Cos}\left[2\theta 1 + (-\delta + \epsilon 1)\omega p\right] + e^{\frac{1}{2}(3\epsilon 1^2+4\delta(\epsilon 1+\epsilon 2))\sigma^2} \\
&\text{Cos}\left[\theta 1 - \theta 2 + \frac{1}{2}(\epsilon 1 - \epsilon 2)\omega p\right] - e^{\frac{1}{2}(3\epsilon 1^2+4\delta(\epsilon 1+\epsilon 2))\sigma^2} \alpha \text{Cos}\left[\theta 1 - \theta 2 + \frac{1}{2}(\epsilon 1 - \epsilon 2)\omega p\right] - \\
&2e^{\frac{1}{2}(3\delta^2+2\delta\epsilon 2+2\epsilon 1(2\epsilon 1+\epsilon 2))\sigma^2} \text{Cos}\left[\theta 2 + \frac{1}{2}(-\delta + \epsilon 2)\omega p\right] + 2e^{\frac{1}{2}(3\delta^2+2\delta\epsilon 2+2\epsilon 1(2\epsilon 1+\epsilon 2))\sigma^2} \alpha \\
&\text{Cos}\left[\theta 2 + \frac{1}{2}(-\delta + \epsilon 2)\omega p\right] + e^{\frac{1}{2}(4\delta^2+3\epsilon 1^2+4\epsilon 1\epsilon 2)\sigma^2} \text{Cos}\left[\theta 1 + \theta 2 + \frac{1}{2}(-2\delta + \epsilon 1 + \epsilon 2)\omega p\right] - \\
&\left. e^{\frac{1}{2}(4\delta^2+3\epsilon 1^2+4\epsilon 1\epsilon 2)\sigma^2} \alpha \text{Cos}\left[\theta 1 + \theta 2 + \frac{1}{2}(-2\delta + \epsilon 1 + \epsilon 2)\omega p\right] \right)
\end{aligned}$$

$$\begin{aligned}
\ln[*]:= \text{P2s}\mu[\delta\_ , \alpha\_ , \sigma\_ , \omega p\_ , \epsilon 1\_ , \epsilon 2\_ , \theta 1\_ , \theta 2\_ ] &:= \frac{1}{8(1+\alpha)} e^{-\frac{1}{2}(4\delta^2+4\epsilon 1^2+2\epsilon 1\epsilon 2+\epsilon 2^2)\sigma^2} \\
&\left( 2e^{\frac{1}{2}(4\delta^2+4\epsilon 1^2+2\epsilon 1\epsilon 2+\epsilon 2^2)\sigma^2} + 2e^{\frac{1}{2}(8\delta\epsilon 1+2\epsilon 1\epsilon 2+\epsilon 2^2)\sigma^2} \alpha + 2e^{\frac{1}{2}(4\delta^2+4\epsilon 1^2+2\epsilon 1\epsilon 2+\epsilon 2^2)\sigma^2} \alpha + \right. \\
&2e^{\frac{1}{2}(3\delta^2+2\delta\epsilon 1+3\epsilon 1^2+2\epsilon 1\epsilon 2+\epsilon 2^2)\sigma^2} (1+3\alpha) \text{Cos}\left[\theta 1 + \frac{1}{2}(-\delta + \epsilon 1)\omega p\right] + \\
&2e^{\frac{1}{2}(4\delta^2+4\epsilon 1^2+2\epsilon 1\epsilon 2+\epsilon 2^2)\sigma^2} \alpha \text{Cos}\left[2\theta 1 + (-\delta + \epsilon 1)\omega p\right] + e^{\frac{1}{2}(3\epsilon 1^2+4\delta(\epsilon 1+\epsilon 2))\sigma^2} \\
&\text{Cos}\left[\theta 1 - \theta 2 + \frac{1}{2}(\epsilon 1 - \epsilon 2)\omega p\right] - e^{\frac{1}{2}(3\epsilon 1^2+4\delta(\epsilon 1+\epsilon 2))\sigma^2} \alpha \text{Cos}\left[\theta 1 - \theta 2 + \frac{1}{2}(\epsilon 1 - \epsilon 2)\omega p\right] + \\
&2e^{\frac{1}{2}(3\delta^2+2\delta\epsilon 2+2\epsilon 1(2\epsilon 1+\epsilon 2))\sigma^2} \text{Cos}\left[\theta 2 + \frac{1}{2}(-\delta + \epsilon 2)\omega p\right] - 2e^{\frac{1}{2}(3\delta^2+2\delta\epsilon 2+2\epsilon 1(2\epsilon 1+\epsilon 2))\sigma^2} \alpha \\
&\text{Cos}\left[\theta 2 + \frac{1}{2}(-\delta + \epsilon 2)\omega p\right] + e^{\frac{1}{2}(4\delta^2+3\epsilon 1^2+4\epsilon 1\epsilon 2)\sigma^2} \text{Cos}\left[\theta 1 + \theta 2 + \frac{1}{2}(-2\delta + \epsilon 1 + \epsilon 2)\omega p\right] - \\
&\left. e^{\frac{1}{2}(4\delta^2+3\epsilon 1^2+4\epsilon 1\epsilon 2)\sigma^2} \alpha \text{Cos}\left[\theta 1 + \theta 2 + \frac{1}{2}(-2\delta + \epsilon 1 + \epsilon 2)\omega p\right] \right)
\end{aligned}$$

$$\begin{aligned}
\ln[*]:= \text{Pcs}\mu[\delta\_ , \alpha\_ , \sigma\_ , \omega p\_ , \epsilon 1\_ , \epsilon 2\_ , \theta 1\_ , \theta 2\_ ] &:= \frac{1}{4(1+\alpha)} e^{-\frac{1}{2}(8\delta^2-8\delta\epsilon 1+5\epsilon 1^2+2\epsilon 1\epsilon 2+\epsilon 2^2)\sigma^2} \\
&\left( 2e^{\frac{1}{2}(8\delta^2-8\delta\epsilon 1+5\epsilon 1^2+2\epsilon 1\epsilon 2+\epsilon 2^2)\sigma^2} + 2e^{\frac{1}{2}(8\delta^2-8\delta\epsilon 1+5\epsilon 1^2+2\epsilon 1\epsilon 2+\epsilon 2^2)\sigma^2} \alpha - 2e^{\frac{1}{2}(4\delta^2+(\epsilon 1+\epsilon 2)^2)\sigma^2} \alpha - \right. \\
&2e^{\frac{1}{2}(8\delta^2-8\delta\epsilon 1+5\epsilon 1^2+2\epsilon 1\epsilon 2+\epsilon 2^2)\sigma^2} \alpha \text{Cos}\left[2\theta 1 + (-\delta + \epsilon 1)\omega p\right] + e^{2(\delta^2-\delta\epsilon 1+\epsilon 1^2+\delta\epsilon 2)\sigma^2} (-1+\alpha) \\
&\text{Cos}\left[\theta 1 - \theta 2 + \frac{1}{2}(\epsilon 1 - \epsilon 2)\omega p\right] - e^{2(\delta^2+(\delta-\epsilon 1)^2+\epsilon 1\epsilon 2)\sigma^2} \text{Cos}\left[\theta 1 + \theta 2 + \frac{1}{2}(-2\delta + \epsilon 1 + \epsilon 2)\omega p\right] + \\
&\left. e^{2(\delta^2+(\delta-\epsilon 1)^2+\epsilon 1\epsilon 2)\sigma^2} \alpha \text{Cos}\left[\theta 1 + \theta 2 + \frac{1}{2}(-2\delta + \epsilon 1 + \epsilon 2)\omega p\right] \right)
\end{aligned}$$

## Noisy

$$\begin{aligned}
\ln[*]:= \text{P1s}\mu\eta[\delta\_ , \alpha\_ , \sigma\_ , \omega\rho\_ , \eta\epsilon\_ , \eta\theta\_ ] := & \frac{1}{4+4\alpha} + \frac{e^{-\frac{8\delta^2\sigma^2+\eta\theta^2(4+8\eta\epsilon^2\sigma^2)+\eta\epsilon^2(1+2\eta\epsilon^2\sigma^2)\omega\rho^2}{4+8\eta\epsilon^2\sigma^2}}}{8(1+\alpha)\sqrt{1+2\eta\epsilon^2\sigma^2}} + \\
& \alpha \left( \frac{1}{4+4\alpha} - \frac{e^{-\frac{8\delta^2\sigma^2+\eta\theta^2(4+8\eta\epsilon^2\sigma^2)+\eta\epsilon^2(1+2\eta\epsilon^2\sigma^2)\omega\rho^2}{4+8\eta\epsilon^2\sigma^2}}}{8(1+\alpha)\sqrt{1+2\eta\epsilon^2\sigma^2}} + \frac{e^{-\frac{2\delta^2\sigma^2}{1+4\eta\epsilon^2\sigma^2}}}{(4+4\alpha)\sqrt{1+4\eta\epsilon^2\sigma^2}} \right) + \\
& \frac{e^{-2\eta\theta^2-\frac{\eta\epsilon^2\omega\rho^2}{2}} \left( -e^{\eta\theta^2+\frac{\eta\epsilon^2\omega\rho^2}{4}} (-1+\alpha) + 2\alpha\sqrt{1+2\eta\epsilon^2\sigma^2} \right) \text{Cos}[\delta\omega\rho]}{8(1+\alpha)\sqrt{1+2\eta\epsilon^2\sigma^2}} - \\
& \frac{e^{-\frac{4\delta^2\sigma^2+4\eta\theta^2(1+\eta\epsilon^2\sigma^2)+\eta\epsilon^2\omega\rho^2}{8+8\eta\epsilon^2\sigma^2}} \text{Cos}\left[\frac{\delta\omega\rho}{2+2\eta\epsilon^2\sigma^2}\right]}{2\sqrt{1+\eta\epsilon^2\sigma^2}}
\end{aligned}$$

$$\begin{aligned}
\ln[*]:= \text{P2s}\mu\eta[\delta\_ , \alpha\_ , \sigma\_ , \omega\rho\_ , \eta\epsilon\_ , \eta\theta\_ ] := & \frac{1}{4+4\alpha} + \frac{e^{-\frac{8\delta^2\sigma^2+\eta\theta^2(4+8\eta\epsilon^2\sigma^2)+\eta\epsilon^2(1+2\eta\epsilon^2\sigma^2)\omega\rho^2}{4+8\eta\epsilon^2\sigma^2}}}{8(1+\alpha)\sqrt{1+2\eta\epsilon^2\sigma^2}} + \\
& \alpha \left( \frac{1}{4+4\alpha} - \frac{e^{-\frac{8\delta^2\sigma^2+\eta\theta^2(4+8\eta\epsilon^2\sigma^2)+\eta\epsilon^2(1+2\eta\epsilon^2\sigma^2)\omega\rho^2}{4+8\eta\epsilon^2\sigma^2}}}{8(1+\alpha)\sqrt{1+2\eta\epsilon^2\sigma^2}} + \frac{e^{-\frac{2\delta^2\sigma^2}{1+4\eta\epsilon^2\sigma^2}}}{(4+4\alpha)\sqrt{1+4\eta\epsilon^2\sigma^2}} \right) + \\
& \frac{e^{-2\eta\theta^2-\frac{\eta\epsilon^2\omega\rho^2}{2}} \left( -e^{\eta\theta^2+\frac{\eta\epsilon^2\omega\rho^2}{4}} (-1+\alpha) + 2\alpha\sqrt{1+2\eta\epsilon^2\sigma^2} \right) \text{Cos}[\delta\omega\rho]}{8(1+\alpha)\sqrt{1+2\eta\epsilon^2\sigma^2}} + \\
& \frac{e^{-\frac{4\delta^2\sigma^2+4\eta\theta^2(1+\eta\epsilon^2\sigma^2)+\eta\epsilon^2\omega\rho^2}{8+8\eta\epsilon^2\sigma^2}} \text{Cos}\left[\frac{\delta\omega\rho}{2+2\eta\epsilon^2\sigma^2}\right]}{2\sqrt{1+\eta\epsilon^2\sigma^2}}
\end{aligned}$$

$$\begin{aligned}
\ln[*]:= \text{Pcs}\mu\eta[\delta\_ , \alpha\_ , \sigma\_ , \omega\rho\_ , \eta\epsilon\_ , \eta\theta\_ ] := & \frac{1}{2+2\alpha} - \frac{e^{-\frac{8\delta^2\sigma^2+\eta\theta^2(4+8\eta\epsilon^2\sigma^2)+\eta\epsilon^2(1+2\eta\epsilon^2\sigma^2)\omega\rho^2}{4+8\eta\epsilon^2\sigma^2}}}{4(1+\alpha)\sqrt{1+2\eta\epsilon^2\sigma^2}} + \\
& \alpha \left( \frac{1}{2+2\alpha} + \frac{e^{-\frac{8\delta^2\sigma^2+\eta\theta^2(4+8\eta\epsilon^2\sigma^2)+\eta\epsilon^2(1+2\eta\epsilon^2\sigma^2)\omega\rho^2}{4+8\eta\epsilon^2\sigma^2}}}{4(1+\alpha)\sqrt{1+2\eta\epsilon^2\sigma^2}} - \frac{e^{-\frac{2\delta^2\sigma^2}{1+4\eta\epsilon^2\sigma^2}}}{(2+2\alpha)\sqrt{1+4\eta\epsilon^2\sigma^2}} \right) + \\
& \frac{e^{-2\eta\theta^2-\frac{\eta\epsilon^2\omega\rho^2}{2}} \left( e^{\eta\theta^2+\frac{\eta\epsilon^2\omega\rho^2}{4}} (-1+\alpha) - 2\alpha\sqrt{1+2\eta\epsilon^2\sigma^2} \right) \text{Cos}[\delta\omega\rho]}{4(1+\alpha)\sqrt{1+2\eta\epsilon^2\sigma^2}}
\end{aligned}$$

$$\ln[*]:= \text{Fs}\mu\eta[\delta\_ , \alpha\_ , \sigma\_ , \omega\rho\_ , \eta\epsilon\_ , \eta\theta\_ ] := \left( \frac{4e^{-\frac{8\delta^2\sigma^2+\eta\theta^2(4+8\eta\epsilon^2\sigma^2)+\eta\epsilon^2(1+2\eta\epsilon^2\sigma^2)\omega\rho^2}{4+8\eta\epsilon^2\sigma^2}} \delta\sigma^2}{(1+\alpha)\sqrt{1+2\eta\epsilon^2\sigma^2} (4+8\eta\epsilon^2\sigma^2)} \right) +$$

$$\begin{aligned}
& \alpha \left( \frac{4 e^{-\frac{2\delta^2 \sigma^2}{1+4\eta\epsilon^2 \sigma^2}} \delta \sigma^2}{(2+2\alpha)(1+4\eta\epsilon^2 \sigma^2)^{3/2}} - \frac{4 e^{-\frac{8\delta^2 \sigma^2 + \eta\theta^2(4+8\eta\epsilon^2 \sigma^2) + \eta\epsilon^2(1+2\eta\epsilon^2 \sigma^2)\omega p^2}{4+8\eta\epsilon^2 \sigma^2}} \delta \sigma^2}{(1+\alpha)\sqrt{1+2\eta\epsilon^2 \sigma^2}(4+8\eta\epsilon^2 \sigma^2)} \right) - \\
& \left. \frac{e^{-2\eta\theta^2 - \frac{\eta\epsilon^2 \omega p^2}{2}} \left( e^{\eta\theta^2 + \frac{\eta\epsilon^2 \omega p^2}{4}} (-1+\alpha) - 2\alpha\sqrt{1+2\eta\epsilon^2 \sigma^2} \right) \omega p \text{Sin}[\delta \omega p]}{4(1+\alpha)\sqrt{1+2\eta\epsilon^2 \sigma^2}} \right)^2 / \\
& \left( \frac{1}{2+2\alpha} - \frac{e^{-\frac{8\delta^2 \sigma^2 + \eta\theta^2(4+8\eta\epsilon^2 \sigma^2) + \eta\epsilon^2(1+2\eta\epsilon^2 \sigma^2)\omega p^2}{4+8\eta\epsilon^2 \sigma^2}}}{4(1+\alpha)\sqrt{1+2\eta\epsilon^2 \sigma^2}} + \right. \\
& \alpha \left( \frac{1}{2+2\alpha} + \frac{e^{-\frac{8\delta^2 \sigma^2 + \eta\theta^2(4+8\eta\epsilon^2 \sigma^2) + \eta\epsilon^2(1+2\eta\epsilon^2 \sigma^2)\omega p^2}{4+8\eta\epsilon^2 \sigma^2}}}{4(1+\alpha)\sqrt{1+2\eta\epsilon^2 \sigma^2}} - \frac{e^{-\frac{2\delta^2 \sigma^2}{1+4\eta\epsilon^2 \sigma^2}}}{(2+2\alpha)\sqrt{1+4\eta\epsilon^2 \sigma^2}} \right) + \\
& \left. \frac{e^{-2\eta\theta^2 - \frac{\eta\epsilon^2 \omega p^2}{2}} \left( e^{\eta\theta^2 + \frac{\eta\epsilon^2 \omega p^2}{4}} (-1+\alpha) - 2\alpha\sqrt{1+2\eta\epsilon^2 \sigma^2} \right) \text{Cos}[\delta \omega p]}{4(1+\alpha)\sqrt{1+2\eta\epsilon^2 \sigma^2}} \right) + \\
& \left( -\frac{2 e^{-\frac{8\delta^2 \sigma^2 + \eta\theta^2(4+8\eta\epsilon^2 \sigma^2) + \eta\epsilon^2(1+2\eta\epsilon^2 \sigma^2)\omega p^2}{4+8\eta\epsilon^2 \sigma^2}} \delta \sigma^2}{(1+\alpha)\sqrt{1+2\eta\epsilon^2 \sigma^2}(4+8\eta\epsilon^2 \sigma^2)} + \alpha \left( -\frac{4 e^{-\frac{2\delta^2 \sigma^2}{1+4\eta\epsilon^2 \sigma^2}} \delta \sigma^2}{(4+4\alpha)(1+4\eta\epsilon^2 \sigma^2)^{3/2}} + \right. \right. \\
& \left. \left. \frac{2 e^{-\frac{8\delta^2 \sigma^2 + \eta\theta^2(4+8\eta\epsilon^2 \sigma^2) + \eta\epsilon^2(1+2\eta\epsilon^2 \sigma^2)\omega p^2}{4+8\eta\epsilon^2 \sigma^2}} \delta \sigma^2}{(1+\alpha)\sqrt{1+2\eta\epsilon^2 \sigma^2}(4+8\eta\epsilon^2 \sigma^2)} \right) - \frac{4 e^{-\frac{4\delta^2 \sigma^2 + 4\eta\theta^2(1+\eta\epsilon^2 \sigma^2) + \eta\epsilon^2 \omega p^2}{8+8\eta\epsilon^2 \sigma^2}} \delta \sigma^2 \text{Cos}\left[\frac{\delta \omega p}{2+2\eta\epsilon^2 \sigma^2}\right]}{\sqrt{1+\eta\epsilon^2 \sigma^2}(8+8\eta\epsilon^2 \sigma^2)} - \right. \\
& \left. \frac{e^{-2\eta\theta^2 - \frac{\eta\epsilon^2 \omega p^2}{2}} \left( -e^{\eta\theta^2 + \frac{\eta\epsilon^2 \omega p^2}{4}} (-1+\alpha) + 2\alpha\sqrt{1+2\eta\epsilon^2 \sigma^2} \right) \omega p \text{Sin}[\delta \omega p]}{8(1+\alpha)\sqrt{1+2\eta\epsilon^2 \sigma^2}} - \right. \\
& \left. \frac{e^{-\frac{4\delta^2 \sigma^2 + 4\eta\theta^2(1+\eta\epsilon^2 \sigma^2) + \eta\epsilon^2 \omega p^2}{8+8\eta\epsilon^2 \sigma^2}} \omega p \text{Sin}\left[\frac{\delta \omega p}{2+2\eta\epsilon^2 \sigma^2}\right]}{2\sqrt{1+\eta\epsilon^2 \sigma^2}(2+2\eta\epsilon^2 \sigma^2)} \right)^2 / \left( \frac{1}{4+4\alpha} + \frac{e^{-\frac{8\delta^2 \sigma^2 + \eta\theta^2(4+8\eta\epsilon^2 \sigma^2) + \eta\epsilon^2(1+2\eta\epsilon^2 \sigma^2)\omega p^2}{4+8\eta\epsilon^2 \sigma^2}}}{8(1+\alpha)\sqrt{1+2\eta\epsilon^2 \sigma^2}} + \right. \\
& \alpha \left( \frac{1}{4+4\alpha} - \frac{e^{-\frac{8\delta^2 \sigma^2 + \eta\theta^2(4+8\eta\epsilon^2 \sigma^2) + \eta\epsilon^2(1+2\eta\epsilon^2 \sigma^2)\omega p^2}{4+8\eta\epsilon^2 \sigma^2}}}{8(1+\alpha)\sqrt{1+2\eta\epsilon^2 \sigma^2}} + \frac{e^{-\frac{2\delta^2 \sigma^2}{1+4\eta\epsilon^2 \sigma^2}}}{(4+4\alpha)\sqrt{1+4\eta\epsilon^2 \sigma^2}} \right) + \\
& \left. \frac{e^{-2\eta\theta^2 - \frac{\eta\epsilon^2 \omega p^2}{2}} \left( -e^{\eta\theta^2 + \frac{\eta\epsilon^2 \omega p^2}{4}} (-1+\alpha) + 2\alpha\sqrt{1+2\eta\epsilon^2 \sigma^2} \right) \text{Cos}[\delta \omega p]}{8(1+\alpha)\sqrt{1+2\eta\epsilon^2 \sigma^2}} \right) +
\end{aligned}$$

$$\begin{aligned}
& \left. \frac{e^{-\frac{4\delta^2\sigma^2+4\eta\theta^2(1+\eta\epsilon^2\sigma^2)+\eta\epsilon^2\omega p^2}{8+8\eta\epsilon^2\sigma^2}} \operatorname{Cos}\left[\frac{\delta\omega p}{2+2\eta\epsilon^2\sigma^2}\right]}{2\sqrt{1+\eta\epsilon^2\sigma^2}} \right) + \\
& \left( -\frac{2e^{-\frac{8\delta^2\sigma^2+\eta\theta^2(4+8\eta\epsilon^2\sigma^2)+\eta\epsilon^2(1+2\eta\epsilon^2\sigma^2)\omega p^2}{4+8\eta\epsilon^2\sigma^2}} \delta\sigma^2}{(1+\alpha)\sqrt{1+2\eta\epsilon^2\sigma^2}(4+8\eta\epsilon^2\sigma^2)} + \alpha \left( -\frac{4e^{-\frac{2\delta^2\sigma^2}{1+4\eta\epsilon^2\sigma^2}} \delta\sigma^2}{(4+4\alpha)(1+4\eta\epsilon^2\sigma^2)^{3/2}} + \right. \right. \\
& \left. \left. \frac{2e^{-\frac{8\delta^2\sigma^2+\eta\theta^2(4+8\eta\epsilon^2\sigma^2)+\eta\epsilon^2(1+2\eta\epsilon^2\sigma^2)\omega p^2}{4+8\eta\epsilon^2\sigma^2}} \delta\sigma^2}{(1+\alpha)\sqrt{1+2\eta\epsilon^2\sigma^2}(4+8\eta\epsilon^2\sigma^2)} \right) + \frac{4e^{-\frac{4\delta^2\sigma^2+4\eta\theta^2(1+\eta\epsilon^2\sigma^2)+\eta\epsilon^2\omega p^2}{8+8\eta\epsilon^2\sigma^2}} \delta\sigma^2 \operatorname{Cos}\left[\frac{\delta\omega p}{2+2\eta\epsilon^2\sigma^2}\right]}{\sqrt{1+\eta\epsilon^2\sigma^2}(8+8\eta\epsilon^2\sigma^2)} - \right. \\
& \left. \frac{e^{-2\eta\theta^2-\frac{\eta\epsilon^2\omega p^2}{2}} \left( -e^{\eta\theta^2+\frac{\eta\epsilon^2\omega p^2}{4}} (-1+\alpha) + 2\alpha\sqrt{1+2\eta\epsilon^2\sigma^2} \right) \omega p \operatorname{Sin}[\delta\omega p]}{8(1+\alpha)\sqrt{1+2\eta\epsilon^2\sigma^2}} + \right. \\
& \left. \frac{e^{-\frac{4\delta^2\sigma^2+4\eta\theta^2(1+\eta\epsilon^2\sigma^2)+\eta\epsilon^2\omega p^2}{8+8\eta\epsilon^2\sigma^2}} \omega p \operatorname{Sin}\left[\frac{\delta\omega p}{2+2\eta\epsilon^2\sigma^2}\right]}{2\sqrt{1+\eta\epsilon^2\sigma^2}(2+2\eta\epsilon^2\sigma^2)} \right)^2 / \left( \frac{1}{4+4\alpha} + \frac{e^{-\frac{8\delta^2\sigma^2+\eta\theta^2(4+8\eta\epsilon^2\sigma^2)+\eta\epsilon^2(1+2\eta\epsilon^2\sigma^2)\omega p^2}{4+8\eta\epsilon^2\sigma^2}}}{8(1+\alpha)\sqrt{1+2\eta\epsilon^2\sigma^2}} + \right. \\
& \left. \alpha \left( \frac{1}{4+4\alpha} - \frac{e^{-\frac{8\delta^2\sigma^2+\eta\theta^2(4+8\eta\epsilon^2\sigma^2)+\eta\epsilon^2(1+2\eta\epsilon^2\sigma^2)\omega p^2}{4+8\eta\epsilon^2\sigma^2}}}{8(1+\alpha)\sqrt{1+2\eta\epsilon^2\sigma^2}} + \frac{e^{-\frac{2\delta^2\sigma^2}{1+4\eta\epsilon^2\sigma^2}}}{(4+4\alpha)\sqrt{1+4\eta\epsilon^2\sigma^2}} \right) + \right. \\
& \left. \frac{e^{-2\eta\theta^2-\frac{\eta\epsilon^2\omega p^2}{2}} \left( -e^{\eta\theta^2+\frac{\eta\epsilon^2\omega p^2}{4}} (-1+\alpha) + 2\alpha\sqrt{1+2\eta\epsilon^2\sigma^2} \right) \operatorname{Cos}[\delta\omega p]}{8(1+\alpha)\sqrt{1+2\eta\epsilon^2\sigma^2}} - \right. \\
& \left. \frac{e^{-\frac{4\delta^2\sigma^2+4\eta\theta^2(1+\eta\epsilon^2\sigma^2)+\eta\epsilon^2\omega p^2}{8+8\eta\epsilon^2\sigma^2}} \operatorname{Cos}\left[\frac{\delta\omega p}{2+2\eta\epsilon^2\sigma^2}\right]}{2\sqrt{1+\eta\epsilon^2\sigma^2}} \right)
\end{aligned}$$

## Frequency-independent photons

### Fixed shift

$$\begin{aligned}
\ln[&]:= \mathbf{P1sind}\mu[\delta\_ , \alpha\_ , \sigma\_ , \omega p\_ , \epsilon 1\_ , \epsilon 2\_ , \theta 1\_ , \theta 2\_ ] := \frac{1}{4(1+\alpha)} \\
& e^{-\frac{1}{2}(2\delta^2+2\epsilon 1^2+\epsilon 2^2)\sigma^2} \left( e^{\frac{1}{2}(\delta^2+\epsilon 1^2)\sigma^2} - e^{\delta\epsilon 1\sigma^2} \operatorname{Cos}\left[\theta 1 + \frac{1}{2}(-\delta+\epsilon 1)\omega p\right] \right) \\
& \left( e^{\frac{1}{2}(\delta^2+\epsilon 1^2+\epsilon 2^2)\sigma^2} (1+\alpha) - 2e^{\frac{1}{2}(2\delta\epsilon 1+\epsilon 2^2)\sigma^2} \alpha \operatorname{Cos}\left[\theta 1 + \frac{1}{2}(-\delta+\epsilon 1)\omega p\right] + \right. \\
& \left. e^{\frac{1}{2}(\epsilon 1^2+2\delta\epsilon 2)\sigma^2} (-1+\alpha) \operatorname{Cos}\left[\theta 2 + \frac{1}{2}(-\delta+\epsilon 2)\omega p\right] \right)
\end{aligned}$$

$$\begin{aligned}
\ln[*]:= & \text{P2sind}\mu[\delta\_ , \alpha\_ , \sigma\_ , \omega p\_ , \epsilon 1\_ , \epsilon 2\_ , \theta 1\_ , \theta 2\_ ] := \frac{1}{4(1+\alpha)} \\
& e^{-\frac{1}{2}(2\delta^2+2\epsilon 1^2+\epsilon 2^2)\sigma^2} \left( e^{\frac{1}{2}(\delta^2+\epsilon 1^2)\sigma^2} + e^{\delta\epsilon 1\sigma^2} \text{Cos}[\theta 1 + \frac{1}{2}(-\delta + \epsilon 1)\omega p] \right) \\
& \left( e^{\frac{1}{2}(\delta^2+\epsilon 1^2+\epsilon 2^2)\sigma^2} (1+\alpha) + 2e^{\frac{1}{2}(2\delta\epsilon 1+\epsilon 2^2)\sigma^2} \alpha \text{Cos}[\theta 1 + \frac{1}{2}(-\delta + \epsilon 1)\omega p] - \right. \\
& \left. e^{\frac{1}{2}(\epsilon 1^2+2\delta\epsilon 2)\sigma^2} (-1+\alpha) \text{Cos}[\theta 2 + \frac{1}{2}(-\delta + \epsilon 2)\omega p] \right)
\end{aligned}$$

$$\begin{aligned}
\ln[*]:= & \text{Pcsind}\mu[\delta\_ , \alpha\_ , \sigma\_ , \omega p\_ , \epsilon 1\_ , \epsilon 2\_ , \theta 1\_ , \theta 2\_ ] := \\
& \frac{1}{4(1+\alpha)} e^{-\frac{1}{2}(4\delta^2-4\delta\epsilon 1+3\epsilon 1^2+\epsilon 2^2)\sigma^2} \left( 2e^{\frac{1}{2}(4\delta^2-4\delta\epsilon 1+3\epsilon 1^2+\epsilon 2^2)\sigma^2} - 2e^{\frac{1}{2}(2\delta^2+\epsilon 1^2+\epsilon 2^2)\sigma^2} \alpha + \right. \\
& 2e^{\frac{1}{2}(4\delta^2-4\delta\epsilon 1+3\epsilon 1^2+\epsilon 2^2)\sigma^2} \alpha - 2e^{\frac{1}{2}(2\delta^2+\epsilon 1^2+\epsilon 2^2)\sigma^2} \alpha \text{Cos}[2\theta 1 + (-\delta + \epsilon 1)\omega p] + \\
& e^{(\delta^2-\delta\epsilon 1+\epsilon 1^2+\delta\epsilon 2)\sigma^2} (-1+\alpha) \text{Cos}[\theta 1 - \theta 2 + \frac{1}{2}(\epsilon 1 - \epsilon 2)\omega p] - \\
& e^{(\delta^2-\delta\epsilon 1+\epsilon 1^2+\delta\epsilon 2)\sigma^2} \text{Cos}[\theta 1 + \theta 2 + \frac{1}{2}(-2\delta + \epsilon 1 + \epsilon 2)\omega p] + \\
& \left. e^{(\delta^2-\delta\epsilon 1+\epsilon 1^2+\delta\epsilon 2)\sigma^2} \alpha \text{Cos}[\theta 1 + \theta 2 + \frac{1}{2}(-2\delta + \epsilon 1 + \epsilon 2)\omega p] \right)
\end{aligned}$$

## Noisy

$$\begin{aligned}
\ln[*]:= & \text{P1sind}\eta[\delta\_ , \alpha\_ , \sigma\_ , \omega p\_ , \eta\epsilon\_ , \eta\theta\_ ] := \\
& \frac{1}{16(1+\alpha)(1+\eta\epsilon^2\sigma^2)^{3/2}\sqrt{1+2\eta\epsilon^2\sigma^2}} e^{-\frac{8\eta\theta^2(1+3\eta\epsilon^2\sigma^2+2\eta\epsilon^4\sigma^4)+4\delta^2\sigma^2(3+6\eta\epsilon^2\sigma^2+2\eta\epsilon^4\sigma^4)+\eta\epsilon^2(1+2\eta\epsilon^2\sigma^2)\omega p^2}{4+12\eta\epsilon^2\sigma^2+8\eta\epsilon^4\sigma^4}} \\
& \left( -2e^{\eta\theta^2+\frac{2\delta^2\sigma^2(1+\eta\epsilon^2\sigma^2)}{1+2\eta\epsilon^2\sigma^2}} (-1+\alpha) \sqrt{1+\eta\epsilon^2\sigma^2} \sqrt{1+2\eta\epsilon^2\sigma^2} \text{Cos}\left[\frac{\delta\omega p}{1+\eta\epsilon^2\sigma^2}\right] + \right. \\
& 4e^{\frac{4\delta^2\sigma^2(2+5\eta\epsilon^2\sigma^2+2\eta\epsilon^4\sigma^4)-\eta\epsilon^2\omega p^2}{4+12\eta\epsilon^2\sigma^2+8\eta\epsilon^4\sigma^4}} \alpha (1+\eta\epsilon^2\sigma^2)^{3/2} \text{Cos}\left[\frac{\delta\omega p}{1+2\eta\epsilon^2\sigma^2}\right] + \\
& 2e^{\eta\theta^2+\frac{2\delta^2\sigma^2(1+\eta\epsilon^2\sigma^2)}{1+2\eta\epsilon^2\sigma^2}} \left( \sqrt{1+\eta\epsilon^2\sigma^2} \left( 2e^{\eta\theta^2+\frac{\eta\epsilon^2(4\delta^2\sigma^4+(1+2\eta\epsilon^2\sigma^2)\omega p^2)}{4+12\eta\epsilon^2\sigma^2+8\eta\epsilon^4\sigma^4}} \alpha (1+\eta\epsilon^2\sigma^2) - \right. \right. \\
& \left. \left. (-1+\alpha) \sqrt{1+2\eta\epsilon^2\sigma^2} + 2e^{\frac{4\delta^2\sigma^2+4\eta\theta^2(1+\eta\epsilon^2\sigma^2)+\eta\epsilon^2\omega p^2}{4+4\eta\epsilon^2\sigma^2}} (1+\alpha)(1+\eta\epsilon^2\sigma^2) \sqrt{1+2\eta\epsilon^2\sigma^2} \right) - \right. \\
& \left. \left. 4e^{\frac{4\delta^2\sigma^2+4\eta\theta^2(1+\eta\epsilon^2\sigma^2)+\eta\epsilon^2\omega p^2}{8+8\eta\epsilon^2\sigma^2}} (1+\alpha)(1+\eta\epsilon^2\sigma^2) \sqrt{1+2\eta\epsilon^2\sigma^2} \text{Cos}\left[\frac{\delta\omega p}{2+2\eta\epsilon^2\sigma^2}\right] \right) \right)
\end{aligned}$$

$$\begin{aligned}
\ln[*] := & \text{P2sind}\mu\eta[\delta_-, \alpha_-, \sigma_-, \omega\text{p}_-, \eta\epsilon_-, \eta\theta_-] := \\
& \frac{1}{16 (1 + \alpha) (1 + \eta\epsilon^2 \sigma^2)^{3/2} \sqrt{1 + 2 \eta\epsilon^2 \sigma^2}} e^{-\frac{8 \eta\theta^2 (1 + 3 \eta\epsilon^2 \sigma^2 + 2 \eta\epsilon^4 \sigma^4) + 4 \delta^2 \sigma^2 (3 + 6 \eta\epsilon^2 \sigma^2 + 2 \eta\epsilon^4 \sigma^4) + \eta\epsilon^2 (1 + 2 \eta\epsilon^2 \sigma^2) \omega\text{p}^2}{4 + 12 \eta\epsilon^2 \sigma^2 + 8 \eta\epsilon^4 \sigma^4}} \\
& \left( -2 e^{\frac{\eta\theta^2 + 2 \delta^2 \sigma^2 (1 + \eta\epsilon^2 \sigma^2)}{1 + 2 \eta\epsilon^2 \sigma^2}} (-1 + \alpha) \sqrt{1 + \eta\epsilon^2 \sigma^2} \sqrt{1 + 2 \eta\epsilon^2 \sigma^2} \cos\left[\frac{\delta \omega\text{p}}{1 + \eta\epsilon^2 \sigma^2}\right] + \right. \\
& 4 e^{\frac{4 \delta^2 \sigma^2 (2 + 5 \eta\epsilon^2 \sigma^2 + 2 \eta\epsilon^4 \sigma^4) - \eta\epsilon^2 \omega\text{p}^2}{4 + 12 \eta\epsilon^2 \sigma^2 + 8 \eta\epsilon^4 \sigma^4}} \alpha (1 + \eta\epsilon^2 \sigma^2)^{3/2} \cos\left[\frac{\delta \omega\text{p}}{1 + 2 \eta\epsilon^2 \sigma^2}\right] + \\
& 2 e^{\eta\theta^2 + \frac{2 \delta^2 \sigma^2 (1 + \eta\epsilon^2 \sigma^2)}{1 + 2 \eta\epsilon^2 \sigma^2}} \left( \sqrt{1 + \eta\epsilon^2 \sigma^2} \left( 2 e^{\eta\theta^2 + \frac{\eta\epsilon^2 (4 \delta^2 \sigma^4 + (1 + 2 \eta\epsilon^2 \sigma^2) \omega\text{p}^2)}{4 + 12 \eta\epsilon^2 \sigma^2 + 8 \eta\epsilon^4 \sigma^4}} \alpha (1 + \eta\epsilon^2 \sigma^2) - \right. \right. \\
& \left. \left. (-1 + \alpha) \sqrt{1 + 2 \eta\epsilon^2 \sigma^2} + 2 e^{\frac{4 \delta^2 \sigma^2 + 4 \eta\theta^2 (1 + \eta\epsilon^2 \sigma^2) + \eta\epsilon^2 \omega\text{p}^2}{4 + 4 \eta\epsilon^2 \sigma^2}} (1 + \alpha) (1 + \eta\epsilon^2 \sigma^2) \sqrt{1 + 2 \eta\epsilon^2 \sigma^2} \right) + \right. \\
& \left. \left. 4 e^{\frac{4 \delta^2 \sigma^2 + 4 \eta\theta^2 (1 + \eta\epsilon^2 \sigma^2) + \eta\epsilon^2 \omega\text{p}^2}{8 + 8 \eta\epsilon^2 \sigma^2}} (1 + \alpha) (1 + \eta\epsilon^2 \sigma^2) \sqrt{1 + 2 \eta\epsilon^2 \sigma^2} \cos\left[\frac{\delta \omega\text{p}}{2 + 2 \eta\epsilon^2 \sigma^2}\right] \right) \right)
\end{aligned}$$

$$\begin{aligned}
\ln[*] := & \text{Pcsind}\mu\eta[\delta_-, \alpha_-, \sigma_-, \omega\text{p}_-, \eta\epsilon_-, \eta\theta_-] := \\
& \frac{1}{2 + 2 \alpha} + \frac{\alpha}{2 + 2 \alpha} - \frac{e^{-\frac{4 \delta^2 \sigma^2 + 4 \eta\theta^2 (1 + \eta\epsilon^2 \sigma^2) + \eta\epsilon^2 \omega\text{p}^2}{4 + 4 \eta\epsilon^2 \sigma^2}}}{4 (1 + \alpha) (1 + \eta\epsilon^2 \sigma^2)} + \frac{e^{-\frac{4 \delta^2 \sigma^2 + 4 \eta\theta^2 (1 + \eta\epsilon^2 \sigma^2) + \eta\epsilon^2 \omega\text{p}^2}{4 + 4 \eta\epsilon^2 \sigma^2}} \alpha}{4 (1 + \alpha) (1 + \eta\epsilon^2 \sigma^2)} - \frac{e^{-\frac{\delta^2 \sigma^2}{1 + 2 \eta\epsilon^2 \sigma^2}} \alpha}{(2 + 2 \alpha) \sqrt{1 + 2 \eta\epsilon^2 \sigma^2}} + \\
& \frac{e^{-\frac{4 \delta^2 \sigma^2 + 4 \eta\theta^2 (1 + \eta\epsilon^2 \sigma^2) + \eta\epsilon^2 \omega\text{p}^2}{4 + 4 \eta\epsilon^2 \sigma^2}} (-1 + \alpha) \cos\left[\frac{\delta \omega\text{p}}{1 + \eta\epsilon^2 \sigma^2}\right]}{4 (1 + \alpha) (1 + \eta\epsilon^2 \sigma^2)} - \frac{e^{-\frac{2 \delta^2 \sigma^2 + \eta\theta^2 (4 + 8 \eta\epsilon^2 \sigma^2) + \eta\epsilon^2 \omega\text{p}^2}{2 + 4 \eta\epsilon^2 \sigma^2}} \alpha \cos\left[\frac{\delta \omega\text{p}}{1 + 2 \eta\epsilon^2 \sigma^2}\right]}{2 (1 + \alpha) \sqrt{1 + 2 \eta\epsilon^2 \sigma^2}}
\end{aligned}$$

$$\begin{aligned}
\ln[*] := & \text{Fsind}\mu\eta[\delta_-, \alpha_-, \sigma_-, \omega\text{p}_-, \eta\epsilon_-, \eta\theta_-] := \\
& \left( \frac{2 e^{-\frac{\delta^2 \sigma^2}{1 + 2 \eta\epsilon^2 \sigma^2}} \alpha \delta \sigma^2}{(2 + 2 \alpha) (1 + 2 \eta\epsilon^2 \sigma^2)^{3/2}} + \frac{2 e^{-\frac{4 \delta^2 \sigma^2 + 4 \eta\theta^2 (1 + \eta\epsilon^2 \sigma^2) + \eta\epsilon^2 \omega\text{p}^2}{4 + 4 \eta\epsilon^2 \sigma^2}} \delta \sigma^2}{(1 + \alpha) (1 + \eta\epsilon^2 \sigma^2) (4 + 4 \eta\epsilon^2 \sigma^2)} - \right. \\
& \frac{2 e^{-\frac{4 \delta^2 \sigma^2 + 4 \eta\theta^2 (1 + \eta\epsilon^2 \sigma^2) + \eta\epsilon^2 \omega\text{p}^2}{4 + 4 \eta\epsilon^2 \sigma^2}} \alpha \delta \sigma^2}{(1 + \alpha) (1 + \eta\epsilon^2 \sigma^2) (4 + 4 \eta\epsilon^2 \sigma^2)} - \frac{2 e^{-\frac{4 \delta^2 \sigma^2 + 4 \eta\theta^2 (1 + \eta\epsilon^2 \sigma^2) + \eta\epsilon^2 \omega\text{p}^2}{4 + 4 \eta\epsilon^2 \sigma^2}} (-1 + \alpha) \delta \sigma^2 \cos\left[\frac{\delta \omega\text{p}}{1 + \eta\epsilon^2 \sigma^2}\right]}{(1 + \alpha) (1 + \eta\epsilon^2 \sigma^2) (4 + 4 \eta\epsilon^2 \sigma^2)} + \\
& \frac{2 e^{-\frac{2 \delta^2 \sigma^2 + \eta\theta^2 (4 + 8 \eta\epsilon^2 \sigma^2) + \eta\epsilon^2 \omega\text{p}^2}{2 + 4 \eta\epsilon^2 \sigma^2}} \alpha \delta \sigma^2 \cos\left[\frac{\delta \omega\text{p}}{1 + 2 \eta\epsilon^2 \sigma^2}\right]}{(1 + \alpha) \sqrt{1 + 2 \eta\epsilon^2 \sigma^2} (2 + 4 \eta\epsilon^2 \sigma^2)} - \\
& \frac{e^{-\frac{4 \delta^2 \sigma^2 + 4 \eta\theta^2 (1 + \eta\epsilon^2 \sigma^2) + \eta\epsilon^2 \omega\text{p}^2}{4 + 4 \eta\epsilon^2 \sigma^2}} (-1 + \alpha) \omega\text{p} \sin\left[\frac{\delta \omega\text{p}}{1 + \eta\epsilon^2 \sigma^2}\right]}{4 (1 + \alpha) (1 + \eta\epsilon^2 \sigma^2)^2} + \\
& \left. \frac{e^{-\frac{2 \delta^2 \sigma^2 + \eta\theta^2 (4 + 8 \eta\epsilon^2 \sigma^2) + \eta\epsilon^2 \omega\text{p}^2}{2 + 4 \eta\epsilon^2 \sigma^2}} \alpha \omega\text{p} \sin\left[\frac{\delta \omega\text{p}}{1 + 2 \eta\epsilon^2 \sigma^2}\right]}{2 (1 + \alpha) (1 + 2 \eta\epsilon^2 \sigma^2)^{3/2}} \right)^2 / \\
& \left( \frac{1}{2 + 2 \alpha} + \frac{\alpha}{2 + 2 \alpha} - \frac{e^{-\frac{4 \delta^2 \sigma^2 + 4 \eta\theta^2 (1 + \eta\epsilon^2 \sigma^2) + \eta\epsilon^2 \omega\text{p}^2}{4 + 4 \eta\epsilon^2 \sigma^2}}}{4 (1 + \alpha) (1 + \eta\epsilon^2 \sigma^2)} + \frac{e^{-\frac{4 \delta^2 \sigma^2 + 4 \eta\theta^2 (1 + \eta\epsilon^2 \sigma^2) + \eta\epsilon^2 \omega\text{p}^2}{4 + 4 \eta\epsilon^2 \sigma^2}} \alpha}{4 (1 + \alpha) (1 + \eta\epsilon^2 \sigma^2)} - \frac{e^{-\frac{\delta^2 \sigma^2}{1 + 2 \eta\epsilon^2 \sigma^2}} \alpha}{(2 + 2 \alpha) \sqrt{1 + 2 \eta\epsilon^2 \sigma^2}} + \right.
\end{aligned}$$

$$\begin{aligned}
& \left. \frac{e^{-\frac{4\delta^2\sigma^2+4\eta\theta^2(1+\eta\epsilon^2\sigma^2)+\eta\epsilon^2\omega p^2}{4+4\eta\epsilon^2\sigma^2}}(-1+\alpha)\operatorname{Cos}\left[\frac{\delta\omega p}{1+\eta\epsilon^2\sigma^2}\right] - e^{-\frac{2\delta^2\sigma^2+\eta\theta^2(4+8\eta\epsilon^2\sigma^2)+\eta\epsilon^2\omega p^2}{2+4\eta\epsilon^2\sigma^2}}\alpha\operatorname{Cos}\left[\frac{\delta\omega p}{1+2\eta\epsilon^2\sigma^2}\right]}{4(1+\alpha)(1+\eta\epsilon^2\sigma^2) - 2(1+\alpha)\sqrt{1+2\eta\epsilon^2\sigma^2}} \right) + \\
& \left( 16e^{\frac{8\eta\theta^2(1+3\eta\epsilon^2\sigma^2+2\eta\epsilon^4\sigma^4)+4\delta^2\sigma^2(3+6\eta\epsilon^2\sigma^2+2\eta\epsilon^4\sigma^4)+\eta\epsilon^2(1+2\eta\epsilon^2\sigma^2)\omega p^2}{4+12\eta\epsilon^2\sigma^2+8\eta\epsilon^4\sigma^4}}(1+\alpha)(1+\eta\epsilon^2\sigma^2)^{3/2}\sqrt{1+2\eta\epsilon^2\sigma^2} \right. \\
& \left. - \left( \left( e^{-\frac{8\eta\theta^2(1+3\eta\epsilon^2\sigma^2+2\eta\epsilon^4\sigma^4)+4\delta^2\sigma^2(3+6\eta\epsilon^2\sigma^2+2\eta\epsilon^4\sigma^4)+\eta\epsilon^2(1+2\eta\epsilon^2\sigma^2)\omega p^2}{4+12\eta\epsilon^2\sigma^2+8\eta\epsilon^4\sigma^4}}\delta\sigma^2(3+6\eta\epsilon^2\sigma^2+2\eta\epsilon^4\sigma^4) \right. \right. \right. \\
& \left. \left. \left( -2e^{\eta\theta^2+\frac{2\delta^2\sigma^2(1+\eta\epsilon^2\sigma^2)}{1+2\eta\epsilon^2\sigma^2}}(-1+\alpha)\sqrt{1+\eta\epsilon^2\sigma^2}\sqrt{1+2\eta\epsilon^2\sigma^2}\operatorname{Cos}\left[\frac{\delta\omega p}{1+\eta\epsilon^2\sigma^2}\right] + \right. \right. \right. \\
& \left. \left. \left. 4e^{\frac{4\delta^2\sigma^2(2+5\eta\epsilon^2\sigma^2+2\eta\epsilon^4\sigma^4)-\eta\epsilon^2\omega p^2}{4+12\eta\epsilon^2\sigma^2+8\eta\epsilon^4\sigma^4}}\alpha(1+\eta\epsilon^2\sigma^2)^{3/2}\operatorname{Cos}\left[\frac{\delta\omega p}{1+2\eta\epsilon^2\sigma^2}\right] + \right. \right. \right. \\
& \left. \left. \left. 2e^{\eta\theta^2+\frac{2\delta^2\sigma^2(1+\eta\epsilon^2\sigma^2)}{1+2\eta\epsilon^2\sigma^2}}\left(\sqrt{1+\eta\epsilon^2\sigma^2}\left(2e^{\eta\theta^2+\frac{\eta\epsilon^2(4\delta^2\sigma^4+(1+2\eta\epsilon^2\sigma^2)\omega p^2)}{4+12\eta\epsilon^2\sigma^2+8\eta\epsilon^4\sigma^4}}\alpha(1+\eta\epsilon^2\sigma^2) - \right. \right. \right. \right. \\
& \left. \left. \left. \left. (-1+\alpha)\sqrt{1+2\eta\epsilon^2\sigma^2} + 2e^{\frac{4\delta^2\sigma^2+4\eta\theta^2(1+\eta\epsilon^2\sigma^2)+\eta\epsilon^2\omega p^2}{4+4\eta\epsilon^2\sigma^2}}(1+\alpha) \right. \right. \right. \right. \\
& \left. \left. \left. \left. \left. (1+\eta\epsilon^2\sigma^2)\sqrt{1+2\eta\epsilon^2\sigma^2} \right) + 4e^{\frac{4\delta^2\sigma^2+4\eta\theta^2(1+\eta\epsilon^2\sigma^2)+\eta\epsilon^2\omega p^2}{8+8\eta\epsilon^2\sigma^2}} \right. \right. \right. \right. \\
& \left. \left. \left. \left. \left. (1+\alpha)(1+\eta\epsilon^2\sigma^2)\sqrt{1+2\eta\epsilon^2\sigma^2}\operatorname{Cos}\left[\frac{\delta\omega p}{2+2\eta\epsilon^2\sigma^2}\right] \right) \right) \right) \right) / \\
& \left. \left( 2(1+\alpha)(1+\eta\epsilon^2\sigma^2)^{3/2}\sqrt{1+2\eta\epsilon^2\sigma^2}(4+12\eta\epsilon^2\sigma^2+8\eta\epsilon^4\sigma^4) \right) \right) + \\
& \frac{1}{16(1+\alpha)(1+\eta\epsilon^2\sigma^2)^{3/2}\sqrt{1+2\eta\epsilon^2\sigma^2}} e^{-\frac{8\eta\theta^2(1+3\eta\epsilon^2\sigma^2+2\eta\epsilon^4\sigma^4)+4\delta^2\sigma^2(3+6\eta\epsilon^2\sigma^2+2\eta\epsilon^4\sigma^4)+\eta\epsilon^2(1+2\eta\epsilon^2\sigma^2)\omega p^2}{4+12\eta\epsilon^2\sigma^2+8\eta\epsilon^4\sigma^4}} \\
& \left( \frac{8e^{\eta\theta^2+\frac{2\delta^2\sigma^2(1+\eta\epsilon^2\sigma^2)}{1+2\eta\epsilon^2\sigma^2}}(-1+\alpha)\delta\sigma^2(1+\eta\epsilon^2\sigma^2)^{3/2}\operatorname{Cos}\left[\frac{\delta\omega p}{1+\eta\epsilon^2\sigma^2}\right]}{\sqrt{1+2\eta\epsilon^2\sigma^2}} + \right. \\
& \left( 32e^{\frac{4\delta^2\sigma^2(2+5\eta\epsilon^2\sigma^2+2\eta\epsilon^4\sigma^4)-\eta\epsilon^2\omega p^2}{4+12\eta\epsilon^2\sigma^2+8\eta\epsilon^4\sigma^4}}\alpha\delta\sigma^2(1+\eta\epsilon^2\sigma^2)^{3/2}(2+5\eta\epsilon^2\sigma^2+2\eta\epsilon^4\sigma^4) \right. \\
& \left. \left. \operatorname{Cos}\left[\frac{\delta\omega p}{1+2\eta\epsilon^2\sigma^2}\right] \right) / (4+12\eta\epsilon^2\sigma^2+8\eta\epsilon^4\sigma^4) + \right. \\
& \frac{1}{1+2\eta\epsilon^2\sigma^2} 8e^{\eta\theta^2+\frac{2\delta^2\sigma^2(1+\eta\epsilon^2\sigma^2)}{1+2\eta\epsilon^2\sigma^2}}\delta\sigma^2(1+\eta\epsilon^2\sigma^2)\left(\sqrt{1+\eta\epsilon^2\sigma^2} \right. \\
& \left. \left( 2e^{\eta\theta^2+\frac{\eta\epsilon^2(4\delta^2\sigma^4+(1+2\eta\epsilon^2\sigma^2)\omega p^2)}{4+12\eta\epsilon^2\sigma^2+8\eta\epsilon^4\sigma^4}}\alpha(1+\eta\epsilon^2\sigma^2) - (-1+\alpha)\sqrt{1+2\eta\epsilon^2\sigma^2} + \right. \right. \\
& \left. \left. 2e^{\frac{4\delta^2\sigma^2+4\eta\theta^2(1+\eta\epsilon^2\sigma^2)+\eta\epsilon^2\omega p^2}{4+4\eta\epsilon^2\sigma^2}}(1+\alpha)(1+\eta\epsilon^2\sigma^2)\sqrt{1+2\eta\epsilon^2\sigma^2} \right) + \right. \\
& \left. 4e^{\frac{4\delta^2\sigma^2+4\eta\theta^2(1+\eta\epsilon^2\sigma^2)+\eta\epsilon^2\omega p^2}{8+8\eta\epsilon^2\sigma^2}}(1+\alpha)(1+\eta\epsilon^2\sigma^2)\sqrt{1+2\eta\epsilon^2\sigma^2}\operatorname{Cos}\left[\frac{\delta\omega p}{2+2\eta\epsilon^2\sigma^2}\right] \right) + \\
& \frac{2e^{\eta\theta^2+\frac{2\delta^2\sigma^2(1+\eta\epsilon^2\sigma^2)}{1+2\eta\epsilon^2\sigma^2}}(-1+\alpha)\sqrt{1+2\eta\epsilon^2\sigma^2}\omega p\operatorname{Sin}\left[\frac{\delta\omega p}{1+\eta\epsilon^2\sigma^2}\right]}{\sqrt{1+\eta\epsilon^2\sigma^2}} -
\end{aligned}$$

$$\begin{aligned}
& \frac{4 e^{\frac{4 \delta^2 \sigma^2 (2+5 \eta \epsilon^2 \sigma^2+2 \eta \epsilon^4 \sigma^4)-\eta \epsilon^2 \omega p^2}{4+12 \eta \epsilon^2 \sigma^2+8 \eta \epsilon^4 \sigma^4}} \alpha (1+\eta \epsilon^2 \sigma^2)^{3/2} \omega p \operatorname{Sin}\left[\frac{\delta \omega p}{1+2 \eta \epsilon^2 \sigma^2}\right]}{1+2 \eta \epsilon^2 \sigma^2} + 2 e^{\eta \theta^2+\frac{2 \delta^2 \sigma^2 (1+\eta \epsilon^2 \sigma^2)}{1+2 \eta \epsilon^2 \sigma^2}} \\
& \left( \sqrt{1+\eta \epsilon^2 \sigma^2} \left( \frac{16 e^{\frac{4 \delta^2 \sigma^2+4 \eta \theta^2 (1+\eta \epsilon^2 \sigma^2)+\eta \epsilon^2 \omega p^2}{4+4 \eta \epsilon^2 \sigma^2}} (1+\alpha) \delta \sigma^2 (1+\eta \epsilon^2 \sigma^2) \sqrt{1+2 \eta \epsilon^2 \sigma^2}}{4+4 \eta \epsilon^2 \sigma^2} + \right. \right. \\
& \left. \left. \frac{16 e^{\eta \theta^2+\frac{\eta \epsilon^2 (4 \delta^2 \sigma^4+(1+2 \eta \epsilon^2 \sigma^2) \omega p^2)}{4+12 \eta \epsilon^2 \sigma^2+8 \eta \epsilon^4 \sigma^4}} \alpha \delta \eta \epsilon^2 \sigma^4 (1+\eta \epsilon^2 \sigma^2)}{4+12 \eta \epsilon^2 \sigma^2+8 \eta \epsilon^4 \sigma^4} \right) + \right. \\
& \left. \frac{32 e^{\frac{4 \delta^2 \sigma^2+4 \eta \theta^2 (1+\eta \epsilon^2 \sigma^2)+\eta \epsilon^2 \omega p^2}{8+8 \eta \epsilon^2 \sigma^2}} (1+\alpha) \delta \sigma^2 (1+\eta \epsilon^2 \sigma^2) \sqrt{1+2 \eta \epsilon^2 \sigma^2} \operatorname{Cos}\left[\frac{\delta \omega p}{2+2 \eta \epsilon^2 \sigma^2}\right]}{8+8 \eta \epsilon^2 \sigma^2} - \right. \\
& \left. \left. \frac{4 e^{\frac{4 \delta^2 \sigma^2+4 \eta \theta^2 (1+\eta \epsilon^2 \sigma^2)+\eta \epsilon^2 \omega p^2}{8+8 \eta \epsilon^2 \sigma^2}} (1+\alpha) (1+\eta \epsilon^2 \sigma^2) \sqrt{1+2 \eta \epsilon^2 \sigma^2} \omega p \operatorname{Sin}\left[\frac{\delta \omega p}{2+2 \eta \epsilon^2 \sigma^2}\right]}{2+2 \eta \epsilon^2 \sigma^2} \right) \right) \right) \right)^2 \\
& / \left( -2 e^{\eta \theta^2+\frac{2 \delta^2 \sigma^2 (1+\eta \epsilon^2 \sigma^2)}{1+2 \eta \epsilon^2 \sigma^2}} (-1+\alpha) \sqrt{1+\eta \epsilon^2 \sigma^2} \sqrt{1+2 \eta \epsilon^2 \sigma^2} \operatorname{Cos}\left[\frac{\delta \omega p}{1+\eta \epsilon^2 \sigma^2}\right] + \right. \\
& 4 e^{\frac{4 \delta^2 \sigma^2 (2+5 \eta \epsilon^2 \sigma^2+2 \eta \epsilon^4 \sigma^4)-\eta \epsilon^2 \omega p^2}{4+12 \eta \epsilon^2 \sigma^2+8 \eta \epsilon^4 \sigma^4}} \alpha (1+\eta \epsilon^2 \sigma^2)^{3/2} \operatorname{Cos}\left[\frac{\delta \omega p}{1+2 \eta \epsilon^2 \sigma^2}\right] + \\
& 2 e^{\eta \theta^2+\frac{2 \delta^2 \sigma^2 (1+\eta \epsilon^2 \sigma^2)}{1+2 \eta \epsilon^2 \sigma^2}} \left( \sqrt{1+\eta \epsilon^2 \sigma^2} \left( 2 e^{\eta \theta^2+\frac{\eta \epsilon^2 (4 \delta^2 \sigma^4+(1+2 \eta \epsilon^2 \sigma^2) \omega p^2)}{4+12 \eta \epsilon^2 \sigma^2+8 \eta \epsilon^4 \sigma^4}} \alpha (1+\eta \epsilon^2 \sigma^2) - \right. \right. \\
& \left. \left. (-1+\alpha) \sqrt{1+2 \eta \epsilon^2 \sigma^2} + 2 e^{\frac{4 \delta^2 \sigma^2+4 \eta \theta^2 (1+\eta \epsilon^2 \sigma^2)+\eta \epsilon^2 \omega p^2}{4+4 \eta \epsilon^2 \sigma^2}} (1+\alpha) (1+\eta \epsilon^2 \sigma^2) \sqrt{1+2 \eta \epsilon^2 \sigma^2} \right) + \right. \\
& \left. \left. 4 e^{\frac{4 \delta^2 \sigma^2+4 \eta \theta^2 (1+\eta \epsilon^2 \sigma^2)+\eta \epsilon^2 \omega p^2}{8+8 \eta \epsilon^2 \sigma^2}} (1+\alpha) (1+\eta \epsilon^2 \sigma^2) \sqrt{1+2 \eta \epsilon^2 \sigma^2} \operatorname{Cos}\left[\frac{\delta \omega p}{2+2 \eta \epsilon^2 \sigma^2}\right] \right) \right) + \\
& \left( 16 e^{\frac{8 \eta \theta^2 (1+3 \eta \epsilon^2 \sigma^2+2 \eta \epsilon^4 \sigma^4)+4 \delta^2 \sigma^2 (3+6 \eta \epsilon^2 \sigma^2+2 \eta \epsilon^4 \sigma^4)+\eta \epsilon^2 (1+2 \eta \epsilon^2 \sigma^2) \omega p^2}{4+12 \eta \epsilon^2 \sigma^2+8 \eta \epsilon^4 \sigma^4}} (1+\alpha) (1+\eta \epsilon^2 \sigma^2)^{3/2} \sqrt{1+2 \eta \epsilon^2 \sigma^2} \right. \\
& \left. - \left( \left( e^{-\frac{8 \eta \theta^2 (1+3 \eta \epsilon^2 \sigma^2+2 \eta \epsilon^4 \sigma^4)+4 \delta^2 \sigma^2 (3+6 \eta \epsilon^2 \sigma^2+2 \eta \epsilon^4 \sigma^4)+\eta \epsilon^2 (1+2 \eta \epsilon^2 \sigma^2) \omega p^2}{4+12 \eta \epsilon^2 \sigma^2+8 \eta \epsilon^4 \sigma^4}} \delta \sigma^2 (3+6 \eta \epsilon^2 \sigma^2+2 \eta \epsilon^4 \sigma^4) \right. \right. \right. \\
& \left. \left. \left( -2 e^{\eta \theta^2+\frac{2 \delta^2 \sigma^2 (1+\eta \epsilon^2 \sigma^2)}{1+2 \eta \epsilon^2 \sigma^2}} (-1+\alpha) \sqrt{1+\eta \epsilon^2 \sigma^2} \sqrt{1+2 \eta \epsilon^2 \sigma^2} \operatorname{Cos}\left[\frac{\delta \omega p}{1+\eta \epsilon^2 \sigma^2}\right] + \right. \right. \\
& 4 e^{\frac{4 \delta^2 \sigma^2 (2+5 \eta \epsilon^2 \sigma^2+2 \eta \epsilon^4 \sigma^4)-\eta \epsilon^2 \omega p^2}{4+12 \eta \epsilon^2 \sigma^2+8 \eta \epsilon^4 \sigma^4}} \alpha (1+\eta \epsilon^2 \sigma^2)^{3/2} \operatorname{Cos}\left[\frac{\delta \omega p}{1+2 \eta \epsilon^2 \sigma^2}\right] + \\
& 2 e^{\eta \theta^2+\frac{2 \delta^2 \sigma^2 (1+\eta \epsilon^2 \sigma^2)}{1+2 \eta \epsilon^2 \sigma^2}} \left( \sqrt{1+\eta \epsilon^2 \sigma^2} \left( 2 e^{\eta \theta^2+\frac{\eta \epsilon^2 (4 \delta^2 \sigma^4+(1+2 \eta \epsilon^2 \sigma^2) \omega p^2)}{4+12 \eta \epsilon^2 \sigma^2+8 \eta \epsilon^4 \sigma^4}} \alpha (1+\eta \epsilon^2 \sigma^2) - \right. \right. \\
& \left. \left. (-1+\alpha) \sqrt{1+2 \eta \epsilon^2 \sigma^2} + 2 e^{\frac{4 \delta^2 \sigma^2+4 \eta \theta^2 (1+\eta \epsilon^2 \sigma^2)+\eta \epsilon^2 \omega p^2}{4+4 \eta \epsilon^2 \sigma^2}} (1+\alpha) \right. \right. \\
& \left. \left. (1+\eta \epsilon^2 \sigma^2) \sqrt{1+2 \eta \epsilon^2 \sigma^2} \right) - 4 e^{\frac{4 \delta^2 \sigma^2+4 \eta \theta^2 (1+\eta \epsilon^2 \sigma^2)+\eta \epsilon^2 \omega p^2}{8+8 \eta \epsilon^2 \sigma^2}} \right. \\
& \left. \left. (1+\alpha) (1+\eta \epsilon^2 \sigma^2) \sqrt{1+2 \eta \epsilon^2 \sigma^2} \operatorname{Cos}\left[\frac{\delta \omega p}{2+2 \eta \epsilon^2 \sigma^2}\right] \right) \right) \right) /
\end{aligned}$$

$$\begin{aligned}
& \left( 2 (1 + \alpha) (1 + \eta \epsilon^2 \sigma^2)^{3/2} \sqrt{1 + 2 \eta \epsilon^2 \sigma^2} (4 + 12 \eta \epsilon^2 \sigma^2 + 8 \eta \epsilon^4 \sigma^4) \right) + \\
& \frac{1}{16 (1 + \alpha) (1 + \eta \epsilon^2 \sigma^2)^{3/2} \sqrt{1 + 2 \eta \epsilon^2 \sigma^2}} e^{-\frac{8 \eta \theta^2 (1 + 3 \eta \epsilon^2 \sigma^2 + 2 \eta \epsilon^4 \sigma^4) + 4 \delta^2 \sigma^2 (3 + 6 \eta \epsilon^2 \sigma^2 + 2 \eta \epsilon^4 \sigma^4) + \eta \epsilon^2 (1 + 2 \eta \epsilon^2 \sigma^2) \omega p^2}{4 + 12 \eta \epsilon^2 \sigma^2 + 8 \eta \epsilon^4 \sigma^4}} \\
& \left( -\frac{8 e^{\eta \theta^2 + \frac{2 \delta^2 \sigma^2 (1 + \eta \epsilon^2 \sigma^2)}{1 + 2 \eta \epsilon^2 \sigma^2}} (-1 + \alpha) \delta \sigma^2 (1 + \eta \epsilon^2 \sigma^2)^{3/2} \operatorname{Cos} \left[ \frac{\delta \omega p}{1 + \eta \epsilon^2 \sigma^2} \right]}{\sqrt{1 + 2 \eta \epsilon^2 \sigma^2}} + \right. \\
& \left( 32 e^{\frac{4 \delta^2 \sigma^2 (2 + 5 \eta \epsilon^2 \sigma^2 + 2 \eta \epsilon^4 \sigma^4) - \eta \epsilon^2 \omega p^2}{4 + 12 \eta \epsilon^2 \sigma^2 + 8 \eta \epsilon^4 \sigma^4}} \alpha \delta \sigma^2 (1 + \eta \epsilon^2 \sigma^2)^{3/2} (2 + 5 \eta \epsilon^2 \sigma^2 + 2 \eta \epsilon^4 \sigma^4) \right. \\
& \left. \operatorname{Cos} \left[ \frac{\delta \omega p}{1 + 2 \eta \epsilon^2 \sigma^2} \right] \right) / (4 + 12 \eta \epsilon^2 \sigma^2 + 8 \eta \epsilon^4 \sigma^4) + \\
& \frac{1}{1 + 2 \eta \epsilon^2 \sigma^2} 8 e^{\eta \theta^2 + \frac{2 \delta^2 \sigma^2 (1 + \eta \epsilon^2 \sigma^2)}{1 + 2 \eta \epsilon^2 \sigma^2}} \delta \sigma^2 (1 + \eta \epsilon^2 \sigma^2) \left( \sqrt{1 + \eta \epsilon^2 \sigma^2} \right. \\
& \left( 2 e^{\eta \theta^2 + \frac{\eta \epsilon^2 (4 \delta^2 \sigma^4 + (1 + 2 \eta \epsilon^2 \sigma^2) \omega p^2)}{4 + 12 \eta \epsilon^2 \sigma^2 + 8 \eta \epsilon^4 \sigma^4}} \alpha (1 + \eta \epsilon^2 \sigma^2) - (-1 + \alpha) \sqrt{1 + 2 \eta \epsilon^2 \sigma^2} + \right. \\
& \left. 2 e^{\frac{4 \delta^2 \sigma^2 + 4 \eta \theta^2 (1 + \eta \epsilon^2 \sigma^2) + \eta \epsilon^2 \omega p^2}{4 + 4 \eta \epsilon^2 \sigma^2}} (1 + \alpha) (1 + \eta \epsilon^2 \sigma^2) \sqrt{1 + 2 \eta \epsilon^2 \sigma^2} \right) - \\
& \left. 4 e^{\frac{4 \delta^2 \sigma^2 + 4 \eta \theta^2 (1 + \eta \epsilon^2 \sigma^2) + \eta \epsilon^2 \omega p^2}{8 + 8 \eta \epsilon^2 \sigma^2}} (1 + \alpha) (1 + \eta \epsilon^2 \sigma^2) \sqrt{1 + 2 \eta \epsilon^2 \sigma^2} \operatorname{Cos} \left[ \frac{\delta \omega p}{2 + 2 \eta \epsilon^2 \sigma^2} \right] \right) + \\
& \frac{2 e^{\eta \theta^2 + \frac{2 \delta^2 \sigma^2 (1 + \eta \epsilon^2 \sigma^2)}{1 + 2 \eta \epsilon^2 \sigma^2}} (-1 + \alpha) \sqrt{1 + 2 \eta \epsilon^2 \sigma^2} \omega p \operatorname{Sin} \left[ \frac{\delta \omega p}{1 + \eta \epsilon^2 \sigma^2} \right]}{\sqrt{1 + \eta \epsilon^2 \sigma^2}} - \\
& \frac{4 e^{\frac{4 \delta^2 \sigma^2 (2 + 5 \eta \epsilon^2 \sigma^2 + 2 \eta \epsilon^4 \sigma^4) - \eta \epsilon^2 \omega p^2}{4 + 12 \eta \epsilon^2 \sigma^2 + 8 \eta \epsilon^4 \sigma^4}} \alpha (1 + \eta \epsilon^2 \sigma^2)^{3/2} \omega p \operatorname{Sin} \left[ \frac{\delta \omega p}{1 + 2 \eta \epsilon^2 \sigma^2} \right]}{1 + 2 \eta \epsilon^2 \sigma^2} + 2 e^{\eta \theta^2 + \frac{2 \delta^2 \sigma^2 (1 + \eta \epsilon^2 \sigma^2)}{1 + 2 \eta \epsilon^2 \sigma^2}} \\
& \left( \sqrt{1 + \eta \epsilon^2 \sigma^2} \left( \frac{16 e^{\frac{4 \delta^2 \sigma^2 + 4 \eta \theta^2 (1 + \eta \epsilon^2 \sigma^2) + \eta \epsilon^2 \omega p^2}{4 + 4 \eta \epsilon^2 \sigma^2}} (1 + \alpha) \delta \sigma^2 (1 + \eta \epsilon^2 \sigma^2) \sqrt{1 + 2 \eta \epsilon^2 \sigma^2}}{4 + 4 \eta \epsilon^2 \sigma^2} + \right. \right. \\
& \left. \frac{16 e^{\eta \theta^2 + \frac{\eta \epsilon^2 (4 \delta^2 \sigma^4 + (1 + 2 \eta \epsilon^2 \sigma^2) \omega p^2)}{4 + 12 \eta \epsilon^2 \sigma^2 + 8 \eta \epsilon^4 \sigma^4}} \alpha \delta \eta \epsilon^2 \sigma^4 (1 + \eta \epsilon^2 \sigma^2)}{4 + 12 \eta \epsilon^2 \sigma^2 + 8 \eta \epsilon^4 \sigma^4} \right) - \\
& \left. \frac{32 e^{\frac{4 \delta^2 \sigma^2 + 4 \eta \theta^2 (1 + \eta \epsilon^2 \sigma^2) + \eta \epsilon^2 \omega p^2}{8 + 8 \eta \epsilon^2 \sigma^2}} (1 + \alpha) \delta \sigma^2 (1 + \eta \epsilon^2 \sigma^2) \sqrt{1 + 2 \eta \epsilon^2 \sigma^2} \operatorname{Cos} \left[ \frac{\delta \omega p}{2 + 2 \eta \epsilon^2 \sigma^2} \right]}{8 + 8 \eta \epsilon^2 \sigma^2} + \right. \\
& \left. \left. \frac{4 e^{\frac{4 \delta^2 \sigma^2 + 4 \eta \theta^2 (1 + \eta \epsilon^2 \sigma^2) + \eta \epsilon^2 \omega p^2}{8 + 8 \eta \epsilon^2 \sigma^2}} (1 + \alpha) (1 + \eta \epsilon^2 \sigma^2) \sqrt{1 + 2 \eta \epsilon^2 \sigma^2} \omega p \operatorname{Sin} \left[ \frac{\delta \omega p}{2 + 2 \eta \epsilon^2 \sigma^2} \right]}{2 + 2 \eta \epsilon^2 \sigma^2} \right) \right) \right) \right) \right)^2 \\
& / \left( -2 e^{\eta \theta^2 + \frac{2 \delta^2 \sigma^2 (1 + \eta \epsilon^2 \sigma^2)}{1 + 2 \eta \epsilon^2 \sigma^2}} (-1 + \alpha) \sqrt{1 + \eta \epsilon^2 \sigma^2} \sqrt{1 + 2 \eta \epsilon^2 \sigma^2} \operatorname{Cos} \left[ \frac{\delta \omega p}{1 + \eta \epsilon^2 \sigma^2} \right] + \right. \\
& \left. 4 e^{\frac{4 \delta^2 \sigma^2 (2 + 5 \eta \epsilon^2 \sigma^2 + 2 \eta \epsilon^4 \sigma^4) - \eta \epsilon^2 \omega p^2}{4 + 12 \eta \epsilon^2 \sigma^2 + 8 \eta \epsilon^4 \sigma^4}} \alpha (1 + \eta \epsilon^2 \sigma^2)^{3/2} \operatorname{Cos} \left[ \frac{\delta \omega p}{1 + 2 \eta \epsilon^2 \sigma^2} \right] + \right.
\end{aligned}$$

$$\begin{aligned}
& 2 e^{\eta\theta^2 + \frac{2\delta^2\sigma^2(1+\eta\epsilon^2\sigma^2)}{1+2\eta\epsilon^2\sigma^2}} \left( \sqrt{1+\eta\epsilon^2\sigma^2} \left( 2 e^{\eta\theta^2 + \frac{\eta\epsilon^2(4\delta^2\sigma^4 + (1+2\eta\epsilon^2\sigma^2)\omega p^2)}{4+12\eta\epsilon^2\sigma^2+8\eta\epsilon^4\sigma^4}} \alpha (1+\eta\epsilon^2\sigma^2) - \right. \right. \\
& \quad \left. \left. (-1+\alpha) \sqrt{1+2\eta\epsilon^2\sigma^2} + 2 e^{\frac{4\delta^2\sigma^2+4\eta\theta^2(1+\eta\epsilon^2\sigma^2)+\eta\epsilon^2\omega p^2}{4+4\eta\epsilon^2\sigma^2}} (1+\alpha) (1+\eta\epsilon^2\sigma^2) \sqrt{1+2\eta\epsilon^2\sigma^2} \right) - \right. \\
& \quad \left. \left. 4 e^{\frac{4\delta^2\sigma^2+4\eta\theta^2(1+\eta\epsilon^2\sigma^2)+\eta\epsilon^2\omega p^2}{8+8\eta\epsilon^2\sigma^2}} (1+\alpha) (1+\eta\epsilon^2\sigma^2) \sqrt{1+2\eta\epsilon^2\sigma^2} \cos\left[\frac{\delta\omega p}{2+2\eta\epsilon^2\sigma^2}\right] \right) \right)
\end{aligned}$$

## MZ2d

### Mode-correlated noise

#### Frequency-entangled photons

##### Fixed shift

$$\ln[*]:= \text{P1d}[\delta\_ , \alpha\_ , \sigma\_ , \omega p\_ , \epsilon\_ , \theta\_ ] := \frac{1}{8} \left( e^{-2(\delta-\epsilon)^2\sigma^2} \left( -1 + 2 e^{2(\delta-\epsilon)^2\sigma^2} + \alpha \right) - (1+\alpha) \cos[2\theta + (-\delta + \epsilon)\omega p] \right)$$

$$\ln[*]:= \text{P2d}[\delta\_ , \alpha\_ , \sigma\_ , \omega p\_ , \epsilon\_ , \theta\_ ] := \frac{1}{8} \left( e^{-2(\delta-\epsilon)^2\sigma^2} \left( -1 + 2 e^{2(\delta-\epsilon)^2\sigma^2} + \alpha \right) - (1+\alpha) \cos[2\theta + (-\delta + \epsilon)\omega p] \right)$$

$$\ln[*]:= \text{Pcd}[\delta\_ , \alpha\_ , \sigma\_ , \omega p\_ , \epsilon\_ , \theta\_ ] := \frac{1}{4} \left( 2 - e^{-2(\delta-\epsilon)^2\sigma^2} \left( -1 + \alpha \right) + (1+\alpha) \cos[2\theta + (-\delta + \epsilon)\omega p] \right)$$

##### Noisy

$$\ln[*]:= \text{P1d}\eta[\delta\_ , \alpha\_ , \sigma\_ , \omega p\_ , \eta\epsilon\_ , \eta\theta\_ ] := \frac{1}{8} \left( 2 - \frac{e^{-\frac{2\delta^2\sigma^2}{1+4\eta\epsilon^2\sigma^2}} (1-\alpha)}{\sqrt{1+4\eta\epsilon^2\sigma^2}} - e^{-2\eta\theta^2 - \frac{\eta\epsilon^2\omega p^2}{2}} (1+\alpha) \cos[\delta\omega p] \right)$$

$$\ln[*]:= \text{P2d}\eta[\delta\_ , \alpha\_ , \sigma\_ , \omega p\_ , \eta\epsilon\_ , \eta\theta\_ ] := \frac{1}{8} \left( 2 - \frac{e^{-\frac{2\delta^2\sigma^2}{1+4\eta\epsilon^2\sigma^2}} (1-\alpha)}{\sqrt{1+4\eta\epsilon^2\sigma^2}} - e^{-2\eta\theta^2 - \frac{\eta\epsilon^2\omega p^2}{2}} (1+\alpha) \cos[\delta\omega p] \right)$$

$$\ln[*]:= \text{Pcd}\eta[\delta\_ , \alpha\_ , \sigma\_ , \omega p\_ , \eta\epsilon\_ , \eta\theta\_ ] := \frac{1}{4} \left( 2 + \frac{e^{-\frac{2\delta^2\sigma^2}{1+4\eta\epsilon^2\sigma^2}} (1-\alpha)}{\sqrt{1+4\eta\epsilon^2\sigma^2}} + e^{-2\eta\theta^2 - \frac{\eta\epsilon^2\omega p^2}{2}} (1+\alpha) \cos[\delta\omega p] \right)$$

$$\begin{aligned}
\ln[*]:= & \text{Fd}\eta[\delta\_ , \alpha\_ , \sigma\_ , \omega p\_ , \eta\epsilon\_ , \eta\theta\_ ] := \\
& - \left( \left( -4 e^{2\eta\theta^2 + \frac{\eta\epsilon^2 \omega p^2}{2}} (-1 + \alpha) \delta \sigma^2 + e^{\frac{2\delta^2 \sigma^2}{1+4\eta\epsilon^2 \sigma^2}} (1 + \alpha) (1 + 4\eta\epsilon^2 \sigma^2)^{3/2} \omega p \text{Sin}[\delta \omega p] \right)^2 / \right. \\
& \left( (1 + 4\eta\epsilon^2 \sigma^2) \left( e^{2\eta\theta^2 + \frac{\eta\epsilon^2 \omega p^2}{2}} \left( -(-1 + \alpha) \sqrt{1 + 4\eta\epsilon^2 \sigma^2} + e^{\frac{2\delta^2 \sigma^2}{1+4\eta\epsilon^2 \sigma^2}} (2 + 8\eta\epsilon^2 \sigma^2) \right) + \right. \right. \\
& \left. \left. e^{\frac{2\delta^2 \sigma^2}{1+4\eta\epsilon^2 \sigma^2}} (1 + \alpha) (1 + 4\eta\epsilon^2 \sigma^2) \text{Cos}[\delta \omega p] \right) \right) \\
& \left( -e^{2\eta\theta^2 + \frac{\eta\epsilon^2 \omega p^2}{2}} \left( (-1 + \alpha) \sqrt{1 + 4\eta\epsilon^2 \sigma^2} + e^{\frac{2\delta^2 \sigma^2}{1+4\eta\epsilon^2 \sigma^2}} (2 + 8\eta\epsilon^2 \sigma^2) \right) + \right. \\
& \left. \left. e^{\frac{2\delta^2 \sigma^2}{1+4\eta\epsilon^2 \sigma^2}} (1 + \alpha) (1 + 4\eta\epsilon^2 \sigma^2) \text{Cos}[\delta \omega p] \right) \right) \Big)
\end{aligned}$$

## Frequency-independent photons

### Fixed shift

$$\ln[*]:= \text{P1dind}[\delta\_ , \alpha\_ , \sigma\_ , \omega p\_ , \epsilon\_ , \theta\_ ] := \frac{1}{8} \left( 2 + e^{-(\delta-\epsilon)^2 \sigma^2} (-1 + \alpha - (1 + \alpha) \text{Cos}[2\theta + (-\delta + \epsilon) \omega p] \right)$$

$$\ln[*]:= \text{P2dind}[\delta\_ , \alpha\_ , \sigma\_ , \omega p\_ , \epsilon\_ , \theta\_ ] := \frac{1}{8} \left( 2 + e^{-(\delta-\epsilon)^2 \sigma^2} (-1 + \alpha - (1 + \alpha) \text{Cos}[2\theta + (-\delta + \epsilon) \omega p] \right)$$

$$\ln[*]:= \text{Pcdind}[\delta\_ , \alpha\_ , \sigma\_ , \omega p\_ , \epsilon\_ , \theta\_ ] := \frac{1}{4} \left( 2 + e^{-(\delta-\epsilon)^2 \sigma^2} (1 - \alpha + (1 + \alpha) \text{Cos}[2\theta + (-\delta + \epsilon) \omega p] \right)$$

### Noisy

$$\begin{aligned}
\ln[*]:= & \text{P1dind}\eta[\delta\_ , \alpha\_ , \sigma\_ , \omega p\_ , \eta\epsilon\_ , \eta\theta\_ ] := \\
& \frac{e^{-\frac{2\delta^2 \sigma^2 + \eta\theta^2 (4+8\eta\epsilon^2 \sigma^2) + \eta\epsilon^2 \omega p^2}{2+4\eta\epsilon^2 \sigma^2}} \left( e^{2\eta\theta^2 + \frac{\eta\epsilon^2 \omega p^2}{2+4\eta\epsilon^2 \sigma^2}} \left( -1 + \alpha + 2 e^{\frac{\delta^2 \sigma^2}{1+2\eta\epsilon^2 \sigma^2}} \sqrt{1 + 2\eta\epsilon^2 \sigma^2} \right) - (1 + \alpha) \text{Cos}\left[\frac{\delta \omega p}{1+2\eta\epsilon^2 \sigma^2}\right] \right)}{8 \sqrt{1 + 2\eta\epsilon^2 \sigma^2}}
\end{aligned}$$

$$\begin{aligned}
\ln[*]:= & \text{P2dind}\eta[\delta\_ , \alpha\_ , \sigma\_ , \omega p\_ , \eta\epsilon\_ , \eta\theta\_ ] := \\
& \frac{e^{-\frac{2\delta^2 \sigma^2 + \eta\theta^2 (4+8\eta\epsilon^2 \sigma^2) + \eta\epsilon^2 \omega p^2}{2+4\eta\epsilon^2 \sigma^2}} \left( e^{2\eta\theta^2 + \frac{\eta\epsilon^2 \omega p^2}{2+4\eta\epsilon^2 \sigma^2}} \left( -1 + \alpha + 2 e^{\frac{\delta^2 \sigma^2}{1+2\eta\epsilon^2 \sigma^2}} \sqrt{1 + 2\eta\epsilon^2 \sigma^2} \right) - (1 + \alpha) \text{Cos}\left[\frac{\delta \omega p}{1+2\eta\epsilon^2 \sigma^2}\right] \right)}{8 \sqrt{1 + 2\eta\epsilon^2 \sigma^2}}
\end{aligned}$$

$$\begin{aligned}
\ln[*]:= & \text{Pcdind}\eta[\delta\_ , \alpha\_ , \sigma\_ , \omega p\_ , \eta\epsilon\_ , \eta\theta\_ ] := \\
& \frac{e^{-\frac{2\delta^2 \sigma^2 + \eta\theta^2 (4+8\eta\epsilon^2 \sigma^2) + \eta\epsilon^2 \omega p^2}{2+4\eta\epsilon^2 \sigma^2}} \left( e^{2\eta\theta^2 + \frac{\eta\epsilon^2 \omega p^2}{2+4\eta\epsilon^2 \sigma^2}} \left( 1 - \alpha + 2 e^{\frac{\delta^2 \sigma^2}{1+2\eta\epsilon^2 \sigma^2}} \sqrt{1 + 2\eta\epsilon^2 \sigma^2} \right) + (1 + \alpha) \text{Cos}\left[\frac{\delta \omega p}{1+2\eta\epsilon^2 \sigma^2}\right] \right)}{4 \sqrt{1 + 2\eta\epsilon^2 \sigma^2}}
\end{aligned}$$

$$\begin{aligned}
\ln[*]:= & \text{Fdind}\eta[\delta\_ , \alpha\_ , \sigma\_ , \omega p\_ , \eta\epsilon\_ , \eta\theta\_ ] := \\
& - \left( \left( -2 e^{2\eta\theta^2 + \frac{\eta\epsilon^2 \omega p^2}{2+4\eta\epsilon^2 \sigma^2}} (-1 + \alpha) \delta \sigma^2 + (1 + \alpha) \left( 2 \delta \sigma^2 \text{Cos}\left[\frac{\delta \omega p}{1 + 2\eta\epsilon^2 \sigma^2}\right] + \omega p \text{Sin}\left[\frac{\delta \omega p}{1 + 2\eta\epsilon^2 \sigma^2}\right] \right) \right)^2 / \right. \\
& \left( (1 + 2\eta\epsilon^2 \sigma^2)^2 \left( -4 e^{\frac{2\delta^2 \sigma^2 + \eta\theta^2 (4+8\eta\epsilon^2 \sigma^2) + \eta\epsilon^2 \omega p^2}{1+2\eta\epsilon^2 \sigma^2}} (1 + 2\eta\epsilon^2 \sigma^2) + \right. \right. \\
& \left. \left. \left( e^{2\eta\theta^2 + \frac{\eta\epsilon^2 \omega p^2}{2+4\eta\epsilon^2 \sigma^2}} (-1 + \alpha) - (1 + \alpha) \text{Cos}\left[\frac{\delta \omega p}{1 + 2\eta\epsilon^2 \sigma^2}\right] \right)^2 \right) \right) \Big)
\end{aligned}$$

# Mode-uncorrelated noise

## Frequency-entangled photons

### Fixed shift

$$\begin{aligned}
 \ln[*]:= & \text{P1d}\mu[\delta_-, \alpha_-, \sigma_-, \omega p_-, \epsilon 1_-, \epsilon 2_-, \theta 1_-, \theta 2_-] := \\
 & \frac{1}{8} e^{-\frac{1}{2} (4 \delta^2 + (\epsilon 1 + \epsilon 2)^2) \sigma^2} \left( 2 e^{\frac{1}{2} (4 \delta^2 + (\epsilon 1 + \epsilon 2)^2) \sigma^2} + 2 e^{\frac{1}{2} (3 \delta^2 + 2 \delta \epsilon 1 + 2 \epsilon 1 \epsilon 2 + \epsilon 2^2) \sigma^2} (-1 + \alpha) \right. \\
 & \quad \left. \cos\left[\theta 1 + \frac{1}{2} (-\delta + \epsilon 1) \omega p\right] - 2 e^{\frac{1}{2} (4 \delta^2 + (\epsilon 1 + \epsilon 2)^2) \sigma^2} \alpha \cos\left[2 \theta 1 + (-\delta + \epsilon 1) \omega p\right] - \right. \\
 & \quad \left. e^{2 \delta (\epsilon 1 + \epsilon 2) \sigma^2} \cos\left[\theta 1 - \theta 2 + \frac{1}{2} (\epsilon 1 - \epsilon 2) \omega p\right] + e^{2 \delta (\epsilon 1 + \epsilon 2) \sigma^2} \alpha \cos\left[\theta 1 - \theta 2 + \frac{1}{2} (\epsilon 1 - \epsilon 2) \omega p\right] + \right. \\
 & \quad \left. 2 e^{\frac{1}{2} (3 \delta^2 + \epsilon 1^2 + 2 \delta \epsilon 2 + 2 \epsilon 1 \epsilon 2) \sigma^2} \cos\left[\theta 2 + \frac{1}{2} (-\delta + \epsilon 2) \omega p\right] - \right. \\
 & \quad \left. 2 e^{\frac{1}{2} (3 \delta^2 + \epsilon 1^2 + 2 \delta \epsilon 2 + 2 \epsilon 1 \epsilon 2) \sigma^2} \alpha \cos\left[\theta 2 + \frac{1}{2} (-\delta + \epsilon 2) \omega p\right] - e^{2 (\delta^2 + \epsilon 1 \epsilon 2) \sigma^2} \right. \\
 & \quad \left. \cos\left[\theta 1 + \theta 2 + \frac{1}{2} (-2 \delta + \epsilon 1 + \epsilon 2) \omega p\right] + e^{2 (\delta^2 + \epsilon 1 \epsilon 2) \sigma^2} \alpha \cos\left[\theta 1 + \theta 2 + \frac{1}{2} (-2 \delta + \epsilon 1 + \epsilon 2) \omega p\right] \right)
 \end{aligned}$$

$$\begin{aligned}
 \ln[*]:= & \text{P2d}\mu[\delta_-, \alpha_-, \sigma_-, \omega p_-, \epsilon 1_-, \epsilon 2_-, \theta 1_-, \theta 2_-] := \\
 & \frac{1}{8} e^{-\frac{1}{2} (4 \delta^2 + (\epsilon 1 + \epsilon 2)^2) \sigma^2} \left( 2 e^{\frac{1}{2} (4 \delta^2 + (\epsilon 1 + \epsilon 2)^2) \sigma^2} - 2 e^{\frac{1}{2} (3 \delta^2 + 2 \delta \epsilon 1 + 2 \epsilon 1 \epsilon 2 + \epsilon 2^2) \sigma^2} (-1 + \alpha) \right. \\
 & \quad \left. \cos\left[\theta 1 + \frac{1}{2} (-\delta + \epsilon 1) \omega p\right] - 2 e^{\frac{1}{2} (4 \delta^2 + (\epsilon 1 + \epsilon 2)^2) \sigma^2} \alpha \cos\left[2 \theta 1 + (-\delta + \epsilon 1) \omega p\right] - \right. \\
 & \quad \left. e^{2 \delta (\epsilon 1 + \epsilon 2) \sigma^2} \cos\left[\theta 1 - \theta 2 + \frac{1}{2} (\epsilon 1 - \epsilon 2) \omega p\right] + e^{2 \delta (\epsilon 1 + \epsilon 2) \sigma^2} \alpha \cos\left[\theta 1 - \theta 2 + \frac{1}{2} (\epsilon 1 - \epsilon 2) \omega p\right] - \right. \\
 & \quad \left. 2 e^{\frac{1}{2} (3 \delta^2 + \epsilon 1^2 + 2 \delta \epsilon 2 + 2 \epsilon 1 \epsilon 2) \sigma^2} \cos\left[\theta 2 + \frac{1}{2} (-\delta + \epsilon 2) \omega p\right] + \right. \\
 & \quad \left. 2 e^{\frac{1}{2} (3 \delta^2 + \epsilon 1^2 + 2 \delta \epsilon 2 + 2 \epsilon 1 \epsilon 2) \sigma^2} \alpha \cos\left[\theta 2 + \frac{1}{2} (-\delta + \epsilon 2) \omega p\right] - e^{2 (\delta^2 + \epsilon 1 \epsilon 2) \sigma^2} \right. \\
 & \quad \left. \cos\left[\theta 1 + \theta 2 + \frac{1}{2} (-2 \delta + \epsilon 1 + \epsilon 2) \omega p\right] + e^{2 (\delta^2 + \epsilon 1 \epsilon 2) \sigma^2} \alpha \cos\left[\theta 1 + \theta 2 + \frac{1}{2} (-2 \delta + \epsilon 1 + \epsilon 2) \omega p\right] \right)
 \end{aligned}$$

$$\begin{aligned}
 \ln[*]:= & \text{Pcd}\mu[\delta_-, \alpha_-, \sigma_-, \omega p_-, \epsilon 1_-, \epsilon 2_-, \theta 1_-, \theta 2_-] := \\
 & \frac{1}{4} e^{-(4 \delta^2 + (\epsilon 1 + \epsilon 2)^2) \sigma^2} \left( 2 e^{(4 \delta^2 + (\epsilon 1 + \epsilon 2)^2) \sigma^2} + 2 e^{(4 \delta^2 + (\epsilon 1 + \epsilon 2)^2) \sigma^2} \alpha \cos[2 \theta 1 - \delta \omega p + \epsilon 1 \omega p] - \right. \\
 & \quad \left. e^{\frac{1}{2} (2 \delta + \epsilon 1 + \epsilon 2)^2 \sigma^2} (-1 + \alpha) \cos\left[\theta 1 - \theta 2 + \frac{1}{2} (\epsilon 1 - \epsilon 2) \omega p\right] + \right. \\
 & \quad \left. e^{\frac{1}{2} (8 \delta^2 + \epsilon 1^2 + 6 \epsilon 1 \epsilon 2 + \epsilon 2^2) \sigma^2} \cos\left[\theta 1 + \theta 2 + \frac{1}{2} (-2 \delta + \epsilon 1 + \epsilon 2) \omega p\right] - \right. \\
 & \quad \left. e^{\frac{1}{2} (8 \delta^2 + \epsilon 1^2 + 6 \epsilon 1 \epsilon 2 + \epsilon 2^2) \sigma^2} \alpha \cos\left[\theta 1 + \theta 2 + \frac{1}{2} (-2 \delta + \epsilon 1 + \epsilon 2) \omega p\right] \right)
 \end{aligned}$$

## Noisy

$$\ln[*]:= \mathbf{P1d}\mu\eta[\delta\_ , \alpha\_ , \sigma\_ , \omega p\_ , \eta\epsilon\_ , \eta\theta\_ ] := \frac{1}{8 \sqrt{1 + 2 \eta\epsilon^2 \sigma^2}} \\ e^{-\frac{4 \delta^2 \sigma^2 + \eta\theta^2 (4 + 8 \eta\epsilon^2 \sigma^2) + \eta\epsilon^2 (1 + 2 \eta\epsilon^2 \sigma^2) \omega p^2}{2 + 4 \eta\epsilon^2 \sigma^2}} \left( e^{\eta\theta^2 + \frac{\eta\epsilon^2 \omega p^2}{4}} \left( -1 + \alpha + 2 e^{\eta\theta^2 + \frac{2 \delta^2 \sigma^2}{1 + 2 \eta\epsilon^2 \sigma^2} + \frac{\eta\epsilon^2 \omega p^2}{4}} \sqrt{1 + 2 \eta\epsilon^2 \sigma^2} \right) + \right. \\ \left. e^{\frac{2 \delta^2 \sigma^2}{1 + 2 \eta\epsilon^2 \sigma^2}} \left( e^{\eta\theta^2 + \frac{\eta\epsilon^2 \omega p^2}{4}} (-1 + \alpha) - 2 \alpha \sqrt{1 + 2 \eta\epsilon^2 \sigma^2} \right) \cos[\delta \omega p] \right)$$

$$\ln[*]:= \mathbf{P2d}\mu\eta[\delta\_ , \alpha\_ , \sigma\_ , \omega p\_ , \eta\epsilon\_ , \eta\theta\_ ] := \frac{1}{8 \sqrt{1 + 2 \eta\epsilon^2 \sigma^2}} \\ e^{-\frac{4 \delta^2 \sigma^2 + \eta\theta^2 (4 + 8 \eta\epsilon^2 \sigma^2) + \eta\epsilon^2 (1 + 2 \eta\epsilon^2 \sigma^2) \omega p^2}{2 + 4 \eta\epsilon^2 \sigma^2}} \left( e^{\eta\theta^2 + \frac{\eta\epsilon^2 \omega p^2}{4}} \left( -1 + \alpha + 2 e^{\eta\theta^2 + \frac{2 \delta^2 \sigma^2}{1 + 2 \eta\epsilon^2 \sigma^2} + \frac{\eta\epsilon^2 \omega p^2}{4}} \sqrt{1 + 2 \eta\epsilon^2 \sigma^2} \right) + \right. \\ \left. e^{\frac{2 \delta^2 \sigma^2}{1 + 2 \eta\epsilon^2 \sigma^2}} \left( e^{\eta\theta^2 + \frac{\eta\epsilon^2 \omega p^2}{4}} (-1 + \alpha) - 2 \alpha \sqrt{1 + 2 \eta\epsilon^2 \sigma^2} \right) \cos[\delta \omega p] \right)$$

$$\ln[*]:= \mathbf{Pcd}\mu\eta[\delta\_ , \alpha\_ , \sigma\_ , \omega p\_ , \eta\epsilon\_ , \eta\theta\_ ] := \frac{1}{4 \sqrt{1 + 2 \eta\epsilon^2 \sigma^2}} \\ e^{-\frac{4 \delta^2 \sigma^2 + \eta\theta^2 (4 + 8 \eta\epsilon^2 \sigma^2) + \eta\epsilon^2 (1 + 2 \eta\epsilon^2 \sigma^2) \omega p^2}{2 + 4 \eta\epsilon^2 \sigma^2}} \left( e^{\eta\theta^2 + \frac{\eta\epsilon^2 \omega p^2}{4}} \left( 1 - \alpha + 2 e^{\eta\theta^2 + \frac{2 \delta^2 \sigma^2}{1 + 2 \eta\epsilon^2 \sigma^2} + \frac{\eta\epsilon^2 \omega p^2}{4}} \sqrt{1 + 2 \eta\epsilon^2 \sigma^2} \right) - \right. \\ \left. e^{\frac{2 \delta^2 \sigma^2}{1 + 2 \eta\epsilon^2 \sigma^2}} \left( e^{\eta\theta^2 + \frac{\eta\epsilon^2 \omega p^2}{4}} (-1 + \alpha) - 2 \alpha \sqrt{1 + 2 \eta\epsilon^2 \sigma^2} \right) \cos[\delta \omega p] \right)$$

$$\ln[*]:= \mathbf{Fd}\mu\eta[\delta\_ , \alpha\_ , \sigma\_ , \omega p\_ , \eta\epsilon\_ , \eta\theta\_ ] := \left( 4 e^{\eta\theta^2 + \frac{\eta\epsilon^2 \omega p^2}{4}} (-1 + \alpha) \delta \sigma^2 + \right. \\ \left. e^{\frac{2 \delta^2 \sigma^2}{1 + 2 \eta\epsilon^2 \sigma^2}} (1 + 2 \eta\epsilon^2 \sigma^2) \left( e^{\eta\theta^2 + \frac{\eta\epsilon^2 \omega p^2}{4}} (-1 + \alpha) - 2 \alpha \sqrt{1 + 2 \eta\epsilon^2 \sigma^2} \right) \omega p \sin[\delta \omega p] \right)^2 / \\ \left( (1 + 2 \eta\epsilon^2 \sigma^2)^2 \left( e^{\eta\theta^2 + \frac{\eta\epsilon^2 \omega p^2}{4}} \left( 1 - \alpha + 2 e^{\eta\theta^2 + \frac{2 \delta^2 \sigma^2}{1 + 2 \eta\epsilon^2 \sigma^2} + \frac{\eta\epsilon^2 \omega p^2}{4}} \sqrt{1 + 2 \eta\epsilon^2 \sigma^2} \right) - \right. \right. \\ \left. \left. e^{\frac{2 \delta^2 \sigma^2}{1 + 2 \eta\epsilon^2 \sigma^2}} \left( e^{\eta\theta^2 + \frac{\eta\epsilon^2 \omega p^2}{4}} (-1 + \alpha) - 2 \alpha \sqrt{1 + 2 \eta\epsilon^2 \sigma^2} \right) \cos[\delta \omega p] \right) \right. \\ \left. \left( e^{\eta\theta^2 + \frac{\eta\epsilon^2 \omega p^2}{4}} \left( -1 + \alpha + 2 e^{\eta\theta^2 + \frac{2 \delta^2 \sigma^2}{1 + 2 \eta\epsilon^2 \sigma^2} + \frac{\eta\epsilon^2 \omega p^2}{4}} \sqrt{1 + 2 \eta\epsilon^2 \sigma^2} \right) + \right. \right. \\ \left. \left. e^{\frac{2 \delta^2 \sigma^2}{1 + 2 \eta\epsilon^2 \sigma^2}} \left( e^{\eta\theta^2 + \frac{\eta\epsilon^2 \omega p^2}{4}} (-1 + \alpha) - 2 \alpha \sqrt{1 + 2 \eta\epsilon^2 \sigma^2} \right) \cos[\delta \omega p] \right) \right)$$

# Frequency-independent photons

## Fixed shift

$$\begin{aligned}
 \text{In[*]} := & \text{P1dind}\mu[\delta\_ , \alpha\_ , \sigma\_ , \omega\text{p}\_ , \epsilon 1\_ , \epsilon 2\_ , \theta 1\_ , \theta 2\_ ] := \\
 & \frac{1}{8} e^{-\frac{1}{2} (2 (\delta^2 + \epsilon 1^2) + \epsilon 2^2) \sigma^2} \left( 2 e^{\frac{1}{2} (2 (\delta^2 + \epsilon 1^2) + \epsilon 2^2) \sigma^2} - 2 e^{\frac{1}{2} (4 \delta \epsilon 1 + \epsilon 2^2) \sigma^2} \alpha \text{Cos}[2 \theta 1 + (-\delta + \epsilon 1) \omega\text{p}] + \right. \\
 & (-1 + \alpha) \left( 2 e^{\frac{1}{2} ((\delta + \epsilon 1)^2 + \epsilon 2^2) \sigma^2} \text{Cos}\left[\theta 1 + \frac{1}{2} (-\delta + \epsilon 1) \omega\text{p}\right] - \right. \\
 & \left. 2 e^{\frac{1}{2} (\delta^2 + 2 \epsilon 1^2 + 2 \delta \epsilon 2) \sigma^2} \text{Cos}\left[\theta 2 + \frac{1}{2} (-\delta + \epsilon 2) \omega\text{p}\right] + e^{\frac{1}{2} (\epsilon 1^2 + 2 \delta (\epsilon 1 + \epsilon 2)) \sigma^2} \right. \\
 & \left. \left. \left( \text{Cos}\left[\theta 1 - \theta 2 + \frac{1}{2} (\epsilon 1 - \epsilon 2) \omega\text{p}\right] + \text{Cos}\left[\theta 1 + \theta 2 + \frac{1}{2} (-2 \delta + \epsilon 1 + \epsilon 2) \omega\text{p}\right] \right) \right) \right)
 \end{aligned}$$

$$\begin{aligned}
 \text{In[*]} := & \text{P2dind}\mu[\delta\_ , \alpha\_ , \sigma\_ , \omega\text{p}\_ , \epsilon 1\_ , \epsilon 2\_ , \theta 1\_ , \theta 2\_ ] := \\
 & \frac{1}{8} e^{-\frac{1}{2} (2 (\delta^2 + \epsilon 1^2) + \epsilon 2^2) \sigma^2} \left( 2 e^{\frac{1}{2} (2 (\delta^2 + \epsilon 1^2) + \epsilon 2^2) \sigma^2} - 2 e^{\frac{1}{2} (4 \delta \epsilon 1 + \epsilon 2^2) \sigma^2} \alpha \text{Cos}[2 \theta 1 + (-\delta + \epsilon 1) \omega\text{p}] + \right. \\
 & (-1 + \alpha) \left( -2 e^{\frac{1}{2} ((\delta + \epsilon 1)^2 + \epsilon 2^2) \sigma^2} \text{Cos}\left[\theta 1 + \frac{1}{2} (-\delta + \epsilon 1) \omega\text{p}\right] + \right. \\
 & \left. 2 e^{\frac{1}{2} (\delta^2 + 2 \epsilon 1^2 + 2 \delta \epsilon 2) \sigma^2} \text{Cos}\left[\theta 2 + \frac{1}{2} (-\delta + \epsilon 2) \omega\text{p}\right] + e^{\frac{1}{2} (\epsilon 1^2 + 2 \delta (\epsilon 1 + \epsilon 2)) \sigma^2} \right. \\
 & \left. \left. \left( \text{Cos}\left[\theta 1 - \theta 2 + \frac{1}{2} (\epsilon 1 - \epsilon 2) \omega\text{p}\right] + \text{Cos}\left[\theta 1 + \theta 2 + \frac{1}{2} (-2 \delta + \epsilon 1 + \epsilon 2) \omega\text{p}\right] \right) \right) \right)
 \end{aligned}$$

$$\begin{aligned}
 \text{In[*]} := & \text{Pcdind}\mu[\delta\_ , \alpha\_ , \sigma\_ , \omega\text{p}\_ , \epsilon 1\_ , \epsilon 2\_ , \theta 1\_ , \theta 2\_ ] := \frac{1}{4} e^{-\frac{1}{2} (2 (\delta^2 + \epsilon 1^2) + \epsilon 2^2) \sigma^2} \\
 & \left( 2 e^{\frac{\epsilon 2^2 \sigma^2}{2}} \left( e^{(\delta^2 + \epsilon 1^2) \sigma^2} + e^{2 \delta \epsilon 1 \sigma^2} \alpha \text{Cos}[2 \theta 1 + (-\delta + \epsilon 1) \omega\text{p}] \right) - e^{\frac{1}{2} (\epsilon 1^2 + 2 \delta (\epsilon 1 + \epsilon 2)) \sigma^2} \right. \\
 & \left. (-1 + \alpha) \left( \text{Cos}\left[\theta 1 - \theta 2 + \frac{1}{2} (\epsilon 1 - \epsilon 2) \omega\text{p}\right] + \text{Cos}\left[\theta 1 + \theta 2 + \frac{1}{2} (-2 \delta + \epsilon 1 + \epsilon 2) \omega\text{p}\right] \right) \right)
 \end{aligned}$$



$$\ln[*]:= \text{Pcdind}\mu\eta[\delta_-, \alpha_-, \sigma_-, \omega p_-, \eta\epsilon_-, \eta\theta_-] :=$$

$$\frac{1}{4} \left( 2 + \frac{e^{-\frac{4\delta^2\sigma^2+4\eta\theta^2(1+\eta\epsilon^2\sigma^2)+\eta\epsilon^2\omega p^2}{4+4\eta\epsilon^2\sigma^2}}}{1+\eta\epsilon^2\sigma^2} - \frac{e^{-\frac{4\delta^2\sigma^2+4\eta\theta^2(1+\eta\epsilon^2\sigma^2)+\eta\epsilon^2\omega p^2}{4+4\eta\epsilon^2\sigma^2}}}{1+4\eta\epsilon^2\sigma^2+3\eta\epsilon^4\sigma^4} \alpha - \frac{3e^{-\frac{4\delta^2\sigma^2+4\eta\theta^2(1+\eta\epsilon^2\sigma^2)+\eta\epsilon^2\omega p^2}{4+4\eta\epsilon^2\sigma^2}}}{1+4\eta\epsilon^2\sigma^2+3\eta\epsilon^4\sigma^4} \alpha \eta\epsilon^2\sigma^2 - \frac{e^{-\frac{4\delta^2\sigma^2+4\eta\theta^2(1+\eta\epsilon^2\sigma^2)+\eta\epsilon^2\omega p^2}{4+4\eta\epsilon^2\sigma^2}}}{1+\eta\epsilon^2\sigma^2} (-1+\alpha) \text{Cos}\left[\frac{\delta\omega p}{1+\eta\epsilon^2\sigma^2}\right] + \frac{2e^{-\frac{2\delta^2\sigma^2+\eta\theta^2(4+8\eta\epsilon^2\sigma^2)+\eta\epsilon^2\omega p^2}{2+4\eta\epsilon^2\sigma^2}}}{\sqrt{1+2\eta\epsilon^2\sigma^2}} \alpha \text{Cos}\left[\frac{\delta\omega p}{1+2\eta\epsilon^2\sigma^2}\right] + \frac{2e^{-\frac{4\delta^2\sigma^2+4\eta\theta^2(1+\eta\epsilon^2\sigma^2)+\eta\epsilon^2\omega p^2}{8+8\eta\epsilon^2\sigma^2}}}{\sqrt{1+\eta\epsilon^2\sigma^2}} \text{Cos}\left[\frac{\delta\omega p}{2+2\eta\epsilon^2\sigma^2}\right] - \frac{2e^{-\frac{4\delta^2\sigma^2+4\eta\theta^2(1+\eta\epsilon^2\sigma^2)+\eta\epsilon^2\omega p^2}{8+8\eta\epsilon^2\sigma^2}}}{\sqrt{1+\eta\epsilon^2\sigma^2}} \alpha \text{Cos}\left[\frac{\delta\omega p}{2+2\eta\epsilon^2\sigma^2}\right] - \frac{2e^{-\frac{4\delta^2\sigma^2+4\eta\theta^2(1+\eta\epsilon^2\sigma^2)+\eta\epsilon^2\omega p^2}{8+8\eta\epsilon^2\sigma^2}}}{\sqrt{1+5\eta\epsilon^2\sigma^2+4\eta\epsilon^4\sigma^4}} \sqrt{1+4\eta\epsilon^2\sigma^2} \text{Cos}\left[\frac{\delta\omega p}{2+2\eta\epsilon^2\sigma^2}\right] + \frac{2e^{-\frac{4\delta^2\sigma^2+4\eta\theta^2(1+\eta\epsilon^2\sigma^2)+\eta\epsilon^2\omega p^2}{8+8\eta\epsilon^2\sigma^2}}}{\sqrt{1+5\eta\epsilon^2\sigma^2+4\eta\epsilon^4\sigma^4}} \alpha \sqrt{1+4\eta\epsilon^2\sigma^2} \text{Cos}\left[\frac{\delta\omega p}{2+2\eta\epsilon^2\sigma^2}\right] \right)$$

$$\ln[*]:= \text{Fdind}\mu\eta[\delta_-, \alpha_-, \sigma_-, \omega p_-, \eta\epsilon_-, \eta\theta_-] :=$$

$$\left( -\frac{8e^{-\frac{4\delta^2\sigma^2+4\eta\theta^2(1+\eta\epsilon^2\sigma^2)+\eta\epsilon^2\omega p^2}{4+4\eta\epsilon^2\sigma^2}}}{(1+\eta\epsilon^2\sigma^2)(4+4\eta\epsilon^2\sigma^2)} \delta\sigma^2 + \frac{8e^{-\frac{4\delta^2\sigma^2+4\eta\theta^2(1+\eta\epsilon^2\sigma^2)+\eta\epsilon^2\omega p^2}{4+4\eta\epsilon^2\sigma^2}}}{(4+4\eta\epsilon^2\sigma^2)(1+4\eta\epsilon^2\sigma^2+3\eta\epsilon^4\sigma^4)} \alpha\delta\sigma^2 + \frac{24e^{-\frac{4\delta^2\sigma^2+4\eta\theta^2(1+\eta\epsilon^2\sigma^2)+\eta\epsilon^2\omega p^2}{4+4\eta\epsilon^2\sigma^2}}}{(4+4\eta\epsilon^2\sigma^2)(1+4\eta\epsilon^2\sigma^2+3\eta\epsilon^4\sigma^4)} \alpha\delta\eta\epsilon^2\sigma^4 + \frac{8e^{-\frac{4\delta^2\sigma^2+4\eta\theta^2(1+\eta\epsilon^2\sigma^2)+\eta\epsilon^2\omega p^2}{4+4\eta\epsilon^2\sigma^2}}}{(1+\eta\epsilon^2\sigma^2)(4+4\eta\epsilon^2\sigma^2)} (-1+\alpha)\delta\sigma^2 \text{Cos}\left[\frac{\delta\omega p}{1+\eta\epsilon^2\sigma^2}\right] + \frac{8e^{-\frac{2\delta^2\sigma^2+\eta\theta^2(4+8\eta\epsilon^2\sigma^2)+\eta\epsilon^2\omega p^2}{2+4\eta\epsilon^2\sigma^2}}}{\sqrt{1+2\eta\epsilon^2\sigma^2}(2+4\eta\epsilon^2\sigma^2)} \alpha\delta\sigma^2 \text{Cos}\left[\frac{\delta\omega p}{1+2\eta\epsilon^2\sigma^2}\right] - \frac{16e^{-\frac{4\delta^2\sigma^2+4\eta\theta^2(1+\eta\epsilon^2\sigma^2)+\eta\epsilon^2\omega p^2}{8+8\eta\epsilon^2\sigma^2}}}{\sqrt{1+\eta\epsilon^2\sigma^2}(8+8\eta\epsilon^2\sigma^2)} \delta\sigma^2 \text{Cos}\left[\frac{\delta\omega p}{2+2\eta\epsilon^2\sigma^2}\right] + \frac{16e^{-\frac{4\delta^2\sigma^2+4\eta\theta^2(1+\eta\epsilon^2\sigma^2)+\eta\epsilon^2\omega p^2}{8+8\eta\epsilon^2\sigma^2}}}{\sqrt{1+\eta\epsilon^2\sigma^2}(8+8\eta\epsilon^2\sigma^2)} \alpha\delta\sigma^2 \text{Cos}\left[\frac{\delta\omega p}{2+2\eta\epsilon^2\sigma^2}\right] + \frac{16e^{-\frac{4\delta^2\sigma^2+4\eta\theta^2(1+\eta\epsilon^2\sigma^2)+\eta\epsilon^2\omega p^2}{8+8\eta\epsilon^2\sigma^2}}}{(8+8\eta\epsilon^2\sigma^2)\sqrt{1+5\eta\epsilon^2\sigma^2+4\eta\epsilon^4\sigma^4}} \delta\sigma^2 \sqrt{1+4\eta\epsilon^2\sigma^2} \text{Cos}\left[\frac{\delta\omega p}{2+2\eta\epsilon^2\sigma^2}\right] - \frac{16e^{-\frac{4\delta^2\sigma^2+4\eta\theta^2(1+\eta\epsilon^2\sigma^2)+\eta\epsilon^2\omega p^2}{8+8\eta\epsilon^2\sigma^2}}}{(8+8\eta\epsilon^2\sigma^2)\sqrt{1+5\eta\epsilon^2\sigma^2+4\eta\epsilon^4\sigma^4}} \alpha\delta\sigma^2 \sqrt{1+4\eta\epsilon^2\sigma^2} \text{Cos}\left[\frac{\delta\omega p}{2+2\eta\epsilon^2\sigma^2}\right] + \frac{e^{-\frac{4\delta^2\sigma^2+4\eta\theta^2(1+\eta\epsilon^2\sigma^2)+\eta\epsilon^2\omega p^2}{4+4\eta\epsilon^2\sigma^2}}}{(1+\eta\epsilon^2\sigma^2)^2} (-1+\alpha)\omega p \text{Sin}\left[\frac{\delta\omega p}{1+\eta\epsilon^2\sigma^2}\right] - \frac{2e^{-\frac{2\delta^2\sigma^2+\eta\theta^2(4+8\eta\epsilon^2\sigma^2)+\eta\epsilon^2\omega p^2}{2+4\eta\epsilon^2\sigma^2}}}{(1+2\eta\epsilon^2\sigma^2)^{3/2}} \alpha\omega p \text{Sin}\left[\frac{\delta\omega p}{1+2\eta\epsilon^2\sigma^2}\right] \right)$$



$$\begin{aligned}
& \frac{16 e^{-\frac{4 \delta^2 \sigma^2 + 4 \eta \theta^2 (1 + \eta \epsilon^2 \sigma^2) + \eta \epsilon^2 \omega p^2}{8 + 8 \eta \epsilon^2 \sigma^2}} \alpha \delta \sigma^2 \sqrt{1 + 4 \eta \epsilon^2 \sigma^2} \operatorname{Cos}\left[\frac{\delta \omega p}{2 + 2 \eta \epsilon^2 \sigma^2}\right]}{(8 + 8 \eta \epsilon^2 \sigma^2) \sqrt{1 + 5 \eta \epsilon^2 \sigma^2 + 4 \eta \epsilon^4 \sigma^4}} \\
& \frac{e^{-\frac{4 \delta^2 \sigma^2 + 4 \eta \theta^2 (1 + \eta \epsilon^2 \sigma^2) + \eta \epsilon^2 \omega p^2}{4 + 4 \eta \epsilon^2 \sigma^2}} (-1 + \alpha) \omega p \operatorname{Sin}\left[\frac{\delta \omega p}{1 + \eta \epsilon^2 \sigma^2}\right]}{(1 + \eta \epsilon^2 \sigma^2)^2} + \frac{2 e^{-\frac{2 \delta^2 \sigma^2 + \eta \theta^2 (4 + 8 \eta \epsilon^2 \sigma^2) + \eta \epsilon^2 \omega p^2}{2 + 4 \eta \epsilon^2 \sigma^2}} \alpha \omega p \operatorname{Sin}\left[\frac{\delta \omega p}{1 + 2 \eta \epsilon^2 \sigma^2}\right]}{(1 + 2 \eta \epsilon^2 \sigma^2)^{3/2}} + \\
& \frac{2 e^{-\frac{4 \delta^2 \sigma^2 + 4 \eta \theta^2 (1 + \eta \epsilon^2 \sigma^2) + \eta \epsilon^2 \omega p^2}{8 + 8 \eta \epsilon^2 \sigma^2}} \omega p \operatorname{Sin}\left[\frac{\delta \omega p}{2 + 2 \eta \epsilon^2 \sigma^2}\right]}{\sqrt{1 + \eta \epsilon^2 \sigma^2} (2 + 2 \eta \epsilon^2 \sigma^2)} - \frac{2 e^{-\frac{4 \delta^2 \sigma^2 + 4 \eta \theta^2 (1 + \eta \epsilon^2 \sigma^2) + \eta \epsilon^2 \omega p^2}{8 + 8 \eta \epsilon^2 \sigma^2}} \alpha \omega p \operatorname{Sin}\left[\frac{\delta \omega p}{2 + 2 \eta \epsilon^2 \sigma^2}\right]}{\sqrt{1 + \eta \epsilon^2 \sigma^2} (2 + 2 \eta \epsilon^2 \sigma^2)} - \\
& \frac{2 e^{-\frac{4 \delta^2 \sigma^2 + 4 \eta \theta^2 (1 + \eta \epsilon^2 \sigma^2) + \eta \epsilon^2 \omega p^2}{8 + 8 \eta \epsilon^2 \sigma^2}} \sqrt{1 + 4 \eta \epsilon^2 \sigma^2} \omega p \operatorname{Sin}\left[\frac{\delta \omega p}{2 + 2 \eta \epsilon^2 \sigma^2}\right]}{(2 + 2 \eta \epsilon^2 \sigma^2) \sqrt{1 + 5 \eta \epsilon^2 \sigma^2 + 4 \eta \epsilon^4 \sigma^4}} + \\
& \frac{2 e^{-\frac{4 \delta^2 \sigma^2 + 4 \eta \theta^2 (1 + \eta \epsilon^2 \sigma^2) + \eta \epsilon^2 \omega p^2}{8 + 8 \eta \epsilon^2 \sigma^2}} \alpha \sqrt{1 + 4 \eta \epsilon^2 \sigma^2} \omega p \operatorname{Sin}\left[\frac{\delta \omega p}{2 + 2 \eta \epsilon^2 \sigma^2}\right]}{(2 + 2 \eta \epsilon^2 \sigma^2) \sqrt{1 + 5 \eta \epsilon^2 \sigma^2 + 4 \eta \epsilon^4 \sigma^4}} \Bigg)^2 / \\
& \left( 4 \left( 2 - \frac{e^{-\frac{4 \delta^2 \sigma^2 + 4 \eta \theta^2 (1 + \eta \epsilon^2 \sigma^2) + \eta \epsilon^2 \omega p^2}{4 + 4 \eta \epsilon^2 \sigma^2}}}{1 + \eta \epsilon^2 \sigma^2} + \frac{e^{-\frac{4 \delta^2 \sigma^2 + 4 \eta \theta^2 (1 + \eta \epsilon^2 \sigma^2) + \eta \epsilon^2 \omega p^2}{4 + 4 \eta \epsilon^2 \sigma^2}} \alpha}{1 + 4 \eta \epsilon^2 \sigma^2 + 3 \eta \epsilon^4 \sigma^4} + \frac{3 e^{-\frac{4 \delta^2 \sigma^2 + 4 \eta \theta^2 (1 + \eta \epsilon^2 \sigma^2) + \eta \epsilon^2 \omega p^2}{4 + 4 \eta \epsilon^2 \sigma^2}} \alpha \eta \epsilon^2 \sigma^2}{1 + 4 \eta \epsilon^2 \sigma^2 + 3 \eta \epsilon^4 \sigma^4} + \right. \right. \\
& \left. \frac{e^{-\frac{4 \delta^2 \sigma^2 + 4 \eta \theta^2 (1 + \eta \epsilon^2 \sigma^2) + \eta \epsilon^2 \omega p^2}{4 + 4 \eta \epsilon^2 \sigma^2}} (-1 + \alpha) \operatorname{Cos}\left[\frac{\delta \omega p}{1 + \eta \epsilon^2 \sigma^2}\right]}{1 + \eta \epsilon^2 \sigma^2} - \frac{2 e^{-\frac{2 \delta^2 \sigma^2 + \eta \theta^2 (4 + 8 \eta \epsilon^2 \sigma^2) + \eta \epsilon^2 \omega p^2}{2 + 4 \eta \epsilon^2 \sigma^2}} \alpha \operatorname{Cos}\left[\frac{\delta \omega p}{1 + 2 \eta \epsilon^2 \sigma^2}\right]}{\sqrt{1 + 2 \eta \epsilon^2 \sigma^2}} - \right. \\
& \left. \frac{2 e^{-\frac{4 \delta^2 \sigma^2 + 4 \eta \theta^2 (1 + \eta \epsilon^2 \sigma^2) + \eta \epsilon^2 \omega p^2}{8 + 8 \eta \epsilon^2 \sigma^2}} \operatorname{Cos}\left[\frac{\delta \omega p}{2 + 2 \eta \epsilon^2 \sigma^2}\right]}{\sqrt{1 + \eta \epsilon^2 \sigma^2}} + \frac{2 e^{-\frac{4 \delta^2 \sigma^2 + 4 \eta \theta^2 (1 + \eta \epsilon^2 \sigma^2) + \eta \epsilon^2 \omega p^2}{8 + 8 \eta \epsilon^2 \sigma^2}} \alpha \operatorname{Cos}\left[\frac{\delta \omega p}{2 + 2 \eta \epsilon^2 \sigma^2}\right]}{\sqrt{1 + \eta \epsilon^2 \sigma^2}} + \right. \\
& \left. \frac{2 e^{-\frac{4 \delta^2 \sigma^2 + 4 \eta \theta^2 (1 + \eta \epsilon^2 \sigma^2) + \eta \epsilon^2 \omega p^2}{8 + 8 \eta \epsilon^2 \sigma^2}} \sqrt{1 + 4 \eta \epsilon^2 \sigma^2} \operatorname{Cos}\left[\frac{\delta \omega p}{2 + 2 \eta \epsilon^2 \sigma^2}\right]}{\sqrt{1 + 5 \eta \epsilon^2 \sigma^2 + 4 \eta \epsilon^4 \sigma^4}} - \right. \\
& \left. \left. \frac{2 e^{-\frac{4 \delta^2 \sigma^2 + 4 \eta \theta^2 (1 + \eta \epsilon^2 \sigma^2) + \eta \epsilon^2 \omega p^2}{8 + 8 \eta \epsilon^2 \sigma^2}} \alpha \sqrt{1 + 4 \eta \epsilon^2 \sigma^2} \operatorname{Cos}\left[\frac{\delta \omega p}{2 + 2 \eta \epsilon^2 \sigma^2}\right]}{\sqrt{1 + 5 \eta \epsilon^2 \sigma^2 + 4 \eta \epsilon^4 \sigma^4}} \right) \right)
\end{aligned}$$

# Classical correlations

$$\ln[*]:= \text{P1CC}\eta[\delta\_ , \alpha\_ , \sigma\_ , \omega p\_ , \eta\epsilon\_ , \eta\theta\_ ] :=$$

$$\left( e^{-\frac{\delta^2 \sigma^2 (3+2\eta\epsilon^2 \sigma^2) + \eta\theta^2 (4+8\eta\epsilon^2 \sigma^2) + \eta\epsilon^2 \omega p^2}{2+4\eta\epsilon^2 \sigma^2}} \left( e^{\frac{\eta\theta^2 (4+8\eta\epsilon^2 \sigma^2) + \delta^2 (\sigma^2+2\eta\epsilon^2 \sigma^4) + \eta\epsilon^2 \omega p^2}{2+4\eta\epsilon^2 \sigma^2}} \sqrt{1+\eta\epsilon^2 \sigma^2} \left( 1+2 e^{\frac{\delta^2 \sigma^2}{1+2\eta\epsilon^2 \sigma^2}} \sqrt{1+2\eta\epsilon^2 \sigma^2} \right) + \right. \right.$$

$$e^{\frac{\delta^2 \sigma^2}{2}} \sqrt{1+\eta\epsilon^2 \sigma^2} \cos\left[\frac{\delta \omega p}{1+2\eta\epsilon^2 \sigma^2}\right] - 4 e^{\frac{12\eta\theta^2 (1+3\eta\epsilon^2 \sigma^2+2\eta\epsilon^4 \sigma^4) + 4\delta^2 \sigma^2 (2+3\eta\epsilon^2 \sigma^2+2\eta\epsilon^4 \sigma^4) + \eta\epsilon^2 (3+2\eta\epsilon^2 \sigma^2) \omega p^2}{8(1+3\eta\epsilon^2 \sigma^2+2\eta\epsilon^4 \sigma^4)}} \left. \right)$$

$$\sqrt{1+2\eta\epsilon^2 \sigma^2} \cos\left[\frac{\delta \omega p}{2+2\eta\epsilon^2 \sigma^2}\right] \Big) / \left( 8 \sqrt{1+\eta\epsilon^2 \sigma^2} \sqrt{1+2\eta\epsilon^2 \sigma^2} \right)$$

$$\ln[*]:= \text{P2CC}\eta[\delta\_ , \alpha\_ , \sigma\_ , \omega p\_ , \eta\epsilon\_ , \eta\theta\_ ] :=$$

$$\left( e^{-\frac{\delta^2 \sigma^2 (3+2\eta\epsilon^2 \sigma^2) + \eta\theta^2 (4+8\eta\epsilon^2 \sigma^2) + \eta\epsilon^2 \omega p^2}{2+4\eta\epsilon^2 \sigma^2}} \left( e^{\frac{\eta\theta^2 (4+8\eta\epsilon^2 \sigma^2) + \delta^2 (\sigma^2+2\eta\epsilon^2 \sigma^4) + \eta\epsilon^2 \omega p^2}{2+4\eta\epsilon^2 \sigma^2}} \sqrt{1+\eta\epsilon^2 \sigma^2} \left( 1+2 e^{\frac{\delta^2 \sigma^2}{1+2\eta\epsilon^2 \sigma^2}} \sqrt{1+2\eta\epsilon^2 \sigma^2} \right) + \right. \right.$$

$$e^{\frac{\delta^2 \sigma^2}{2}} \sqrt{1+\eta\epsilon^2 \sigma^2} \cos\left[\frac{\delta \omega p}{1+2\eta\epsilon^2 \sigma^2}\right] + 4 e^{\frac{12\eta\theta^2 (1+3\eta\epsilon^2 \sigma^2+2\eta\epsilon^4 \sigma^4) + 4\delta^2 \sigma^2 (2+3\eta\epsilon^2 \sigma^2+2\eta\epsilon^4 \sigma^4) + \eta\epsilon^2 (3+2\eta\epsilon^2 \sigma^2) \omega p^2}{8(1+3\eta\epsilon^2 \sigma^2+2\eta\epsilon^4 \sigma^4)}} \left. \right)$$

$$\sqrt{1+2\eta\epsilon^2 \sigma^2} \cos\left[\frac{\delta \omega p}{2+2\eta\epsilon^2 \sigma^2}\right] \Big) / \left( 8 \sqrt{1+\eta\epsilon^2 \sigma^2} \sqrt{1+2\eta\epsilon^2 \sigma^2} \right)$$

$$\ln[*]:= \text{PcCC}\eta[\delta\_ , \alpha\_ , \sigma\_ , \omega p\_ , \eta\epsilon\_ , \eta\theta\_ ] :=$$

$$\frac{1}{4} \left( 2 - \frac{e^{-\frac{\delta^2 \sigma^2}{1+2\eta\epsilon^2 \sigma^2}}}{\sqrt{1+2\eta\epsilon^2 \sigma^2}} - \frac{e^{-\frac{2\delta^2 \sigma^2 + \eta\theta^2 (4+8\eta\epsilon^2 \sigma^2) + \eta\epsilon^2 \omega p^2}{2+4\eta\epsilon^2 \sigma^2}} \cos\left[\frac{\delta \omega p}{1+2\eta\epsilon^2 \sigma^2}\right]}{\sqrt{1+2\eta\epsilon^2 \sigma^2}} \right)$$

## von Mises distribution

The noisy probabilities calculated in the paper and throughout this notebook assume Gaussian distributions for noise. For  $\theta$  noise, this produces probabilities equivalent to the wrapped Gaussian distribution (see Appendix E).

An alternative circular distribution for  $\theta$  noise is the von Mises distribution, this produces qualitatively the same behaviour but with slight differences in noise dependence.

A reader who wishes to obtain the noisy probabilities with a von Mises distribution may do so by taking the fixed shift probabilities in this notebook, and performing the integral in Eq. (25) replacing the  $\theta$  distribution with

$$\ln[*]:= \text{J}\theta\text{VM}[\theta\_ , \eta\theta\_ ] := \frac{\text{Exp}\left[\frac{\cos[\theta]}{\eta\theta^2}\right]}{2\pi \text{BesselI}\left[\theta, \frac{1}{\eta\theta^2}\right]}$$

and integrating  $\theta$  only between  $-\pi$  and  $\pi$ .

(If  $\epsilon$  noise is also being considered, its Gaussian distribution should remain and  $\epsilon$  integrated between  $-\infty$  and  $\infty$ )

Appendix E also includes comparison between Gaussian and von Mises distributions for  $\theta$  noise for a few limited cases: MZ1, MZ2s, and MZ2d with frequency-entangled photons and mode-correlated noise.

As the noisy probabilities with von Mises have been calculated explicitly for these three cases, they are included below.

(Note all cases here assume no  $\epsilon$  noise, so the  $\eta\epsilon$  variable is absent from these expressions)

## MZ1

$$\text{In[*]}:= \text{P1sing}\eta\text{VM}[\delta\_ , \alpha\_ , \sigma\_ , \omega\text{p}\_ , \eta\theta\_ ] := \frac{1}{2} \left( 1 - \frac{e^{-\frac{1}{2}\delta^2\sigma^2} \text{BesselI}\left[1, \frac{1}{\eta\theta^2}\right] \text{Cos}\left[\frac{\delta\omega\text{p}}{2}\right]}{\text{BesselI}\left[0, \frac{1}{\eta\theta^2}\right]} \right)$$

$$\text{In[*]}:= \text{P2sing}\eta\text{VM}[\delta\_ , \alpha\_ , \sigma\_ , \omega\text{p}\_ , \eta\theta\_ ] := \frac{1}{2} \left( 1 + \frac{e^{-\frac{1}{2}\delta^2\sigma^2} \text{BesselI}\left[1, \frac{1}{\eta\theta^2}\right] \text{Cos}\left[\frac{\delta\omega\text{p}}{2}\right]}{\text{BesselI}\left[0, \frac{1}{\eta\theta^2}\right]} \right)$$

$$\text{In[*]}:= \text{Fsing}\eta\text{VM}[\delta\_ , \alpha\_ , \sigma\_ , \omega\text{p}\_ , \eta\theta\_ ] := \frac{\text{BesselI}\left[1, \frac{1}{\eta\theta^2}\right]^2 \left( 2\delta\sigma^2 \text{Cos}\left[\frac{\delta\omega\text{p}}{2}\right] + \omega\text{p} \text{Sin}\left[\frac{\delta\omega\text{p}}{2}\right] \right)^2}{-4e^{\delta^2\sigma^2} \text{BesselI}\left[0, \frac{1}{\eta\theta^2}\right]^2 + 2\text{BesselI}\left[1, \frac{1}{\eta\theta^2}\right]^2 (1 + \text{Cos}[\delta\omega\text{p}])}$$

## MZ2s

$$\text{In[*]}:= \text{P1s}\eta\text{VM}[\delta\_ , \alpha\_ , \sigma\_ , \omega\text{p}\_ , \eta\theta\_ ] := \frac{1}{8} \left( 2 + e^{-2\delta^2\sigma^2} + \text{Cos}[\delta\omega\text{p}] + \frac{2\text{BesselI}\left[1, \frac{1}{\eta\theta^2}\right] \left( -2e^{-\frac{1}{2}\delta^2\sigma^2} \text{Cos}\left[\frac{\delta\omega\text{p}}{2}\right] - \eta\theta^2 \text{Cos}[\delta\omega\text{p}] \right)}{\text{BesselI}\left[0, \frac{1}{\eta\theta^2}\right]} \right)$$

$$\text{In[*]}:= \text{P2s}\eta\text{VM}[\delta\_ , \alpha\_ , \sigma\_ , \omega\text{p}\_ , \eta\theta\_ ] := \frac{1}{8} \left( 2 + e^{-2\delta^2\sigma^2} + \text{Cos}[\delta\omega\text{p}] + \frac{2\text{BesselI}\left[1, \frac{1}{\eta\theta^2}\right] \left( 2e^{-\frac{1}{2}\delta^2\sigma^2} \text{Cos}\left[\frac{\delta\omega\text{p}}{2}\right] - \eta\theta^2 \text{Cos}[\delta\omega\text{p}] \right)}{\text{BesselI}\left[0, \frac{1}{\eta\theta^2}\right]} \right)$$

$$\text{In[*]}:= \text{Pcs}\eta\text{VM}[\delta\_ , \alpha\_ , \sigma\_ , \omega\text{p}\_ , \eta\theta\_ ] := \frac{1}{4} \left( 2 - e^{-2\delta^2\sigma^2} - \text{Cos}[\delta\omega\text{p}] + \frac{2\eta\theta^2 \text{BesselI}\left[1, \frac{1}{\eta\theta^2}\right] \text{Cos}[\delta\omega\text{p}]}{\text{BesselI}\left[0, \frac{1}{\eta\theta^2}\right]} \right)$$

$$\text{In[*]} := \text{Fs}\eta\text{VM}[\delta_-, \alpha_-, \sigma_-, \omega p_-, \eta\theta_-] :=$$

$$\frac{1}{8} \left( \frac{2 \left( 4 e^{-2 \delta^2 \sigma^2} \delta \sigma^2 + \omega p \text{Sin}[\delta \omega p] - \frac{2 \eta \theta^2 \omega p \text{BesselI}\left[1, \frac{1}{\eta \theta^2}\right] \text{Sin}[\delta \omega p]}{\text{BesselI}\left[\theta, \frac{1}{\eta \theta^2}\right]} \right)^2}{-2 + e^{-2 \delta^2 \sigma^2} + \text{Cos}[\delta \omega p] - \frac{2 \eta \theta^2 \text{BesselI}\left[1, \frac{1}{\eta \theta^2}\right] \text{Cos}[\delta \omega p]}{\text{BesselI}\left[\theta, \frac{1}{\eta \theta^2}\right]}} + \right.$$

$$\left. \frac{\left( 4 e^{-2 \delta^2 \sigma^2} \delta \sigma^2 + \omega p \text{Sin}[\delta \omega p] + \frac{2 e^{-\frac{1}{2} \delta^2 \sigma^2} \text{BesselI}\left[1, \frac{1}{\eta \theta^2}\right] \left( 2 \delta \sigma^2 \text{Cos}\left[\frac{\delta \omega p}{2}\right] + \omega p \left( \text{Sin}\left[\frac{\delta \omega p}{2}\right] - e^{\frac{\delta^2 \sigma^2}{2}} \eta \theta^2 \text{Sin}[\delta \omega p] \right) \right)}{\text{BesselI}\left[\theta, \frac{1}{\eta \theta^2}\right]} \right)^2}{2 + e^{-2 \delta^2 \sigma^2} + \text{Cos}[\delta \omega p] + \frac{2 \text{BesselI}\left[1, \frac{1}{\eta \theta^2}\right] \left( 2 e^{-\frac{1}{2} \delta^2 \sigma^2} \text{Cos}\left[\frac{\delta \omega p}{2}\right] - \eta \theta^2 \text{Cos}[\delta \omega p] \right)}{\text{BesselI}\left[\theta, \frac{1}{\eta \theta^2}\right]}} + \right.$$

$$\left. \frac{\left( 4 e^{-2 \delta^2 \sigma^2} \delta \sigma^2 + \omega p \text{Sin}[\delta \omega p] - \frac{2 e^{-\frac{1}{2} \delta^2 \sigma^2} \text{BesselI}\left[1, \frac{1}{\eta \theta^2}\right] \left( 2 \delta \sigma^2 \text{Cos}\left[\frac{\delta \omega p}{2}\right] + \omega p \left( \text{Sin}\left[\frac{\delta \omega p}{2}\right] + e^{\frac{\delta^2 \sigma^2}{2}} \eta \theta^2 \text{Sin}[\delta \omega p] \right) \right)}{\text{BesselI}\left[\theta, \frac{1}{\eta \theta^2}\right]} \right)^2}{2 + e^{-2 \delta^2 \sigma^2} + \text{Cos}[\delta \omega p] + \frac{2 \text{BesselI}\left[1, \frac{1}{\eta \theta^2}\right] \left( -2 e^{-\frac{1}{2} \delta^2 \sigma^2} \text{Cos}\left[\frac{\delta \omega p}{2}\right] - \eta \theta^2 \text{Cos}[\delta \omega p] \right)}{\text{BesselI}\left[\theta, \frac{1}{\eta \theta^2}\right]}} \right)$$

## MZ2d

$$\text{In[*]} := \text{P1d}\eta\text{VM}[\delta_-, \alpha_-, \sigma_-, \omega p_-, \eta\theta_-] :=$$

$$\frac{1}{8} \left( 2 + e^{-2 \delta^2 \sigma^2} (-1 + \alpha) - (1 + \alpha) \text{Cos}[\delta \omega p] + \frac{2 (1 + \alpha) \eta \theta^2 \text{BesselI}\left[1, \frac{1}{\eta \theta^2}\right] \text{Cos}[\delta \omega p]}{\text{BesselI}\left[\theta, \frac{1}{\eta \theta^2}\right]} \right)$$

$$\text{In[*]} := \text{P2d}\eta\text{VM}[\delta_-, \alpha_-, \sigma_-, \omega p_-, \eta\theta_-] :=$$

$$\frac{1}{8} \left( 2 + e^{-2 \delta^2 \sigma^2} (-1 + \alpha) - (1 + \alpha) \text{Cos}[\delta \omega p] + \frac{2 (1 + \alpha) \eta \theta^2 \text{BesselI}\left[1, \frac{1}{\eta \theta^2}\right] \text{Cos}[\delta \omega p]}{\text{BesselI}\left[\theta, \frac{1}{\eta \theta^2}\right]} \right)$$

$$\text{In[*]} := \text{Pcd}\eta\text{VM}[\delta_-, \alpha_-, \sigma_-, \omega p_-, \eta\theta_-] :=$$

$$\frac{1}{4} \left( 2 - e^{-2 \delta^2 \sigma^2} (-1 + \alpha) + (1 + \alpha) \text{Cos}[\delta \omega p] - \frac{2 (1 + \alpha) \eta \theta^2 \text{BesselI}\left[1, \frac{1}{\eta \theta^2}\right] \text{Cos}[\delta \omega p]}{\text{BesselI}\left[\theta, \frac{1}{\eta \theta^2}\right]} \right)$$

$$\begin{aligned}
\text{In[*]} := & \text{Fd}\eta\text{VM}[\delta\_ , \alpha\_ , \sigma\_ , \omega\text{p}\_ , \eta\theta\_ ] := \\
& - \left( \left( -2 e^{2\delta^2\sigma^2} (1 + \alpha) \eta\theta^2 \omega\text{p} \text{BesselI}\left[1, \frac{1}{\eta\theta^2}\right] \text{Sin}[\delta \omega\text{p}] + \text{BesselI}\left[0, \frac{1}{\eta\theta^2}\right] \right. \right. \\
& \quad \left. \left. (-4 (-1 + \alpha) \delta \sigma^2 + e^{2\delta^2\sigma^2} (1 + \alpha) \omega\text{p} \text{Sin}[\delta \omega\text{p}]) \right)^2 / \right. \\
& \quad \left( \left( -2 e^{2\delta^2\sigma^2} (1 + \alpha) \eta\theta^2 \text{BesselI}\left[1, \frac{1}{\eta\theta^2}\right] \text{Cos}[\delta \omega\text{p}] + \text{BesselI}\left[0, \frac{1}{\eta\theta^2}\right] \right. \right. \\
& \quad \left. \left. (1 - 2 e^{2\delta^2\sigma^2} - \alpha + e^{2\delta^2\sigma^2} (1 + \alpha) \text{Cos}[\delta \omega\text{p}]) \right) \left( -2 e^{2\delta^2\sigma^2} (1 + \alpha) \eta\theta^2 \text{BesselI}\left[1, \frac{1}{\eta\theta^2}\right] \right. \right. \\
& \quad \left. \left. \text{Cos}[\delta \omega\text{p}] + \text{BesselI}\left[0, \frac{1}{\eta\theta^2}\right] (1 + 2 e^{2\delta^2\sigma^2} - \alpha + e^{2\delta^2\sigma^2} (1 + \alpha) \text{Cos}[\delta \omega\text{p}]) \right) \right) \right)
\end{aligned}$$

## Adding Loss

This section allows for the generation of lossy probabilities for a given protocol configuration. Loss is represented by  $\gamma$ , the per photon loss rate.

First, run the earlier sections of this notebook to define all the non-lossy expressions.

Choose a protocol and configuration and run the cells for that choice. This will set the generic probability functions equal to the relevant probabilities for your chosen configuration.

Then, lossy expressions can be generated for either bucket detectors (i.e. those detectors that cannot distinguish between photon numbers) or number-resolving detectors.

Choose a detector type, and run the code for that section to generate probabilities and Fisher information.

Probabilities must be generated first before Fisher information, as the latter calls the probability functions.

The code will attempt to simplify the Fisher information expression. Sometimes this can take some time, the “TimeConstraint” parameter ensures simplification will cancel for cases where it takes too long (usually MZ2s cases). Increasing this parameter may allow more complicated simplifications to complete, though this may take some time to evaluate and there is no guarantee the automatic simplification will ever be possible for every configuration.

## Protocol configuration choice

### HOM

#### Frequency-entangled photons

$$\text{In[*]} := \text{P1}[\delta\_ , \alpha\_ , \sigma\_ , \omega\text{p}\_ , \eta\epsilon\_ , \eta\theta\_ ] := \text{P1HOM}\eta[\delta, \alpha, \sigma, \omega\text{p}, \eta\epsilon, \eta\theta]$$

$$\text{In[*]} := \text{P2}[\delta\_ , \alpha\_ , \sigma\_ , \omega\text{p}\_ , \eta\epsilon\_ , \eta\theta\_ ] := \text{P2HOM}\eta[\delta, \alpha, \sigma, \omega\text{p}, \eta\epsilon, \eta\theta]$$

$\text{In[*]}:= \text{Pc}[\delta_, \alpha_, \sigma_, \omega\text{p}__, \eta\epsilon_, \eta\theta_] := \text{PcHOM}\eta[\delta, \alpha, \sigma, \omega\text{p}, \eta\epsilon, \eta\theta]$

## Frequency-independent photons

$\text{P1}[\delta_, \alpha_, \sigma_, \omega\text{p}__, \eta\epsilon_, \eta\theta_] := \text{P1HOM}\text{ind}\eta[\delta, \alpha, \sigma, \omega\text{p}, \eta\epsilon, \eta\theta]$

$\text{P2}[\delta_, \alpha_, \sigma_, \omega\text{p}__, \eta\epsilon_, \eta\theta_] := \text{P2HOM}\text{ind}\eta[\delta, \alpha, \sigma, \omega\text{p}, \eta\epsilon, \eta\theta]$

$\text{Pc}[\delta_, \alpha_, \sigma_, \omega\text{p}__, \eta\epsilon_, \eta\theta_] := \text{PcHOM}\text{ind}\eta[\delta, \alpha, \sigma, \omega\text{p}, \eta\epsilon, \eta\theta]$

## MZ2s

### Mode-correlated noise

#### Frequency-entangled photons

$\text{In[*]}:= \text{P1}[\delta_, \alpha_, \sigma_, \omega\text{p}__, \eta\epsilon_, \eta\theta_] := \text{P1s}\eta[\delta, \alpha, \sigma, \omega\text{p}, \eta\epsilon, \eta\theta]$

$\text{In[*]}:= \text{P2}[\delta_, \alpha_, \sigma_, \omega\text{p}__, \eta\epsilon_, \eta\theta_] := \text{P2s}\eta[\delta, \alpha, \sigma, \omega\text{p}, \eta\epsilon, \eta\theta]$

$\text{In[*]}:= \text{Pc}[\delta_, \alpha_, \sigma_, \omega\text{p}__, \eta\epsilon_, \eta\theta_] := \text{Pcs}\eta[\delta, \alpha, \sigma, \omega\text{p}, \eta\epsilon, \eta\theta]$

#### Frequency-independent photons

$\text{P1}[\delta_, \alpha_, \sigma_, \omega\text{p}__, \eta\epsilon_, \eta\theta_] := \text{P1s}\text{ind}\eta[\delta, \alpha, \sigma, \omega\text{p}, \eta\epsilon, \eta\theta]$

$\text{P2}[\delta_, \alpha_, \sigma_, \omega\text{p}__, \eta\epsilon_, \eta\theta_] := \text{P2s}\text{ind}\eta[\delta, \alpha, \sigma, \omega\text{p}, \eta\epsilon, \eta\theta]$

$\text{Pc}[\delta_, \alpha_, \sigma_, \omega\text{p}__, \eta\epsilon_, \eta\theta_] := \text{Pcs}\text{ind}\eta[\delta, \alpha, \sigma, \omega\text{p}, \eta\epsilon, \eta\theta]$

### Mode-uncorrelated noise

#### Frequency-entangled photons

$\text{P1}[\delta_, \alpha_, \sigma_, \omega\text{p}__, \eta\epsilon_, \eta\theta_] := \text{P1s}\mu\eta[\delta, \alpha, \sigma, \omega\text{p}, \eta\epsilon, \eta\theta]$

$\text{P2}[\delta_, \alpha_, \sigma_, \omega\text{p}__, \eta\epsilon_, \eta\theta_] := \text{P2s}\mu\eta[\delta, \alpha, \sigma, \omega\text{p}, \eta\epsilon, \eta\theta]$

$\text{Pc}[\delta_, \alpha_, \sigma_, \omega\text{p}__, \eta\epsilon_, \eta\theta_] := \text{Pcs}\mu\eta[\delta, \alpha, \sigma, \omega\text{p}, \eta\epsilon, \eta\theta]$

#### Frequency-independent photons

$\text{P1}[\delta_, \alpha_, \sigma_, \omega\text{p}__, \eta\epsilon_, \eta\theta_] := \text{P1s}\text{ind}\mu\eta[\delta, \alpha, \sigma, \omega\text{p}, \eta\epsilon, \eta\theta]$

$\text{P2}[\delta_, \alpha_, \sigma_, \omega\text{p}__, \eta\epsilon_, \eta\theta_] := \text{P2s}\text{ind}\mu\eta[\delta, \alpha, \sigma, \omega\text{p}, \eta\epsilon, \eta\theta]$

$\text{Pc}[\delta_, \alpha_, \sigma_, \omega\text{p}__, \eta\epsilon_, \eta\theta_] := \text{Pcs}\text{ind}\mu\eta[\delta, \alpha, \sigma, \omega\text{p}, \eta\epsilon, \eta\theta]$

## MZ2d

### Mode-correlated noise

#### Frequency-entangled photons

$$\text{In[*]}:= \mathbf{P1}[\delta_, \alpha_, \sigma_, \omega\mathbf{p}__, \eta\epsilon_, \eta\theta_] := \mathbf{P1d}\eta[\delta, \alpha, \sigma, \omega\mathbf{p}, \eta\epsilon, \eta\theta]$$

$$\text{In[*]}:= \mathbf{P2}[\delta_, \alpha_, \sigma_, \omega\mathbf{p}__, \eta\epsilon_, \eta\theta_] := \mathbf{P2d}\eta[\delta, \alpha, \sigma, \omega\mathbf{p}, \eta\epsilon, \eta\theta]$$

$$\text{In[*]}:= \mathbf{Pc}[\delta_, \alpha_, \sigma_, \omega\mathbf{p}__, \eta\epsilon_, \eta\theta_] := \mathbf{Pcd}\eta[\delta, \alpha, \sigma, \omega\mathbf{p}, \eta\epsilon, \eta\theta]$$

#### Frequency-independent photons

$$\text{In[*]}:= \mathbf{P1}[\delta_, \alpha_, \sigma_, \omega\mathbf{p}__, \eta\epsilon_, \eta\theta_] := \mathbf{P1dind}\eta[\delta, \alpha, \sigma, \omega\mathbf{p}, \eta\epsilon, \eta\theta]$$

$$\text{In[*]}:= \mathbf{P2}[\delta_, \alpha_, \sigma_, \omega\mathbf{p}__, \eta\epsilon_, \eta\theta_] := \mathbf{P2dind}\eta[\delta, \alpha, \sigma, \omega\mathbf{p}, \eta\epsilon, \eta\theta]$$

$$\text{In[*]}:= \mathbf{Pc}[\delta_, \alpha_, \sigma_, \omega\mathbf{p}__, \eta\epsilon_, \eta\theta_] := \mathbf{Pcdind}\eta[\delta, \alpha, \sigma, \omega\mathbf{p}, \eta\epsilon, \eta\theta]$$

### Mode-uncorrelated noise

#### Frequency-entangled photons

$$\mathbf{P1}[\delta_, \alpha_, \sigma_, \omega\mathbf{p}__, \eta\epsilon_, \eta\theta_] := \mathbf{P1d}\mu\eta[\delta, \alpha, \sigma, \omega\mathbf{p}, \eta\epsilon, \eta\theta]$$

$$\mathbf{P2}[\delta_, \alpha_, \sigma_, \omega\mathbf{p}__, \eta\epsilon_, \eta\theta_] := \mathbf{P2d}\mu\eta[\delta, \alpha, \sigma, \omega\mathbf{p}, \eta\epsilon, \eta\theta]$$

$$\mathbf{Pc}[\delta_, \alpha_, \sigma_, \omega\mathbf{p}__, \eta\epsilon_, \eta\theta_] := \mathbf{Pcd}\mu\eta[\delta, \alpha, \sigma, \omega\mathbf{p}, \eta\epsilon, \eta\theta]$$

#### Frequency-independent photons

$$\text{In[*]}:= \mathbf{P1}[\delta_, \alpha_, \sigma_, \omega\mathbf{p}__, \eta\epsilon_, \eta\theta_] := \mathbf{P1dind}\mu\eta[\delta, \alpha, \sigma, \omega\mathbf{p}, \eta\epsilon, \eta\theta]$$

$$\text{In[*]}:= \mathbf{P2}[\delta_, \alpha_, \sigma_, \omega\mathbf{p}__, \eta\epsilon_, \eta\theta_] := \mathbf{P2dind}\mu\eta[\delta, \alpha, \sigma, \omega\mathbf{p}, \eta\epsilon, \eta\theta]$$

$$\text{In[*]}:= \mathbf{Pc}[\delta_, \alpha_, \sigma_, \omega\mathbf{p}__, \eta\epsilon_, \eta\theta_] := \mathbf{Pcdind}\mu\eta[\delta, \alpha, \sigma, \omega\mathbf{p}, \eta\epsilon, \eta\theta]$$

# Generate lossy probabilities and Fisher information

## Bucket detectors

### Probabilities

#### generate

```

In[*]:= Pcγ[δ_, α_, σ_, ωp_, ηε_, ηθ_, γ_] := (1 - γ) ^ 2 Pc[δ, α, σ, ωp, ηε, ηθ] // Simplify;
(*coincidence*)

In[*]:= P1γ[δ_, α_, σ_, ωp_, ηε_, ηθ_, γ_] := (1 - γ) ^ 2 P1[δ, α, σ, ωp, ηε, ηθ] + γ (1 - γ)
(2 P1[δ, α, σ, ωp, ηε, ηθ] + Pc[δ, α, σ, ωp, ηε, ηθ]) // Simplify; (*click at D1*)

In[*]:= P2γ[δ_, α_, σ_, ωp_, ηε_, ηθ_, γ_] := (1 - γ) ^ 2 P2[δ, α, σ, ωp, ηε, ηθ] + γ (1 - γ)
(2 P2[δ, α, σ, ωp, ηε, ηθ] + Pc[δ, α, σ, ωp, ηε, ηθ]) // Simplify; (*click at D2*)

In[*]:= P0γ[δ_, α_, σ_, ωp_, ηε_, ηθ_, γ_] := γ ^ 2; (*no clicks*)

```

#### output

```

In[*]:= Pcγ[δ, α, σ, ωp, ηε, ηθ, γ]

In[*]:= P1γ[δ, α, σ, ωp, ηε, ηθ, γ]

In[*]:= P2γ[δ, α, σ, ωp, ηε, ηθ, γ]

In[*]:= P0γ[δ, α, σ, ωp, ηε, ηθ, γ]

```

### Fisher information

#### generate

```

In[*]:= 
$$\frac{D[Pc\gamma[\delta, \alpha, \sigma, \omega p, \eta \epsilon, \eta \theta, \gamma], \delta]^2}{Pc\gamma[\delta, \alpha, \sigma, \omega p, \eta \epsilon, \eta \theta, \gamma]} + \frac{D[P1\gamma[\delta, \alpha, \sigma, \omega p, \eta \epsilon, \eta \theta, \gamma], \delta]^2}{P1\gamma[\delta, \alpha, \sigma, \omega p, \eta \epsilon, \eta \theta, \gamma]} + \frac{D[P2\gamma[\delta, \alpha, \sigma, \omega p, \eta \epsilon, \eta \theta, \gamma], \delta]^2}{P2\gamma[\delta, \alpha, \sigma, \omega p, \eta \epsilon, \eta \theta, \gamma]}$$


In[*]:= Simplify[%, TimeConstraint -> 1];

In[*]:= Fγ[δ_, α_, σ_, ωp_, ηε_, ηθ_, γ_] = %;

```

#### output

```

In[*]:= Fγ[δ, α, σ, ωp, ηε, ηθ, γ]

```

# Number-resolving detectors detectors

## Probabilities

### generate

```

In[*]:= Pcγ[δ_, α_, σ_, ωp_, ηε_, ηθ_, γ_] := (1 - γ) ^ 2 Pc[δ, α, σ, ωp, ηε, ηθ] // Simplify;
(*coincidence*)

In[*]:= P12γ[δ_, α_, σ_, ωp_, ηε_, ηθ_, γ_] := (1 - γ) ^ 2 P1[δ, α, σ, ωp, ηε, ηθ] // Simplify;
(*two clicks at D1*)

In[*]:= P11γ[δ_, α_, σ_, ωp_, ηε_, ηθ_, γ_] :=
  γ (1 - γ) (2 P1[δ, α, σ, ωp, ηε, ηθ] + Pc[δ, α, σ, ωp, ηε, ηθ]) //
  Simplify; (*one click at D1*)

In[*]:= P22γ[δ_, α_, σ_, ωp_, ηε_, ηθ_, γ_] := (1 - γ) ^ 2 P2[δ, α, σ, ωp, ηε, ηθ] // Simplify;
(*two clicks at D2*)

In[*]:= P21γ[δ_, α_, σ_, ωp_, ηε_, ηθ_, γ_] :=
  γ (1 - γ) (2 P2[δ, α, σ, ωp, ηε, ηθ] + Pc[δ, α, σ, ωp, ηε, ηθ]) // Simplify;
(*two clicks at D1*)

In[*]:= P0γ[δ_, α_, σ_, ωp_, ηε_, ηθ_, γ_] := γ ^ 2; (*no clicks*)

```

### output

```

In[*]:= Pcγ[δ, α, σ, ωp, ηε, ηθ, γ]

In[*]:= P12γ[δ, α, σ, ωp, ηε, ηθ, γ]

In[*]:= P11γ[δ, α, σ, ωp, ηε, ηθ, γ]

In[*]:= P22γ[δ, α, σ, ωp, ηε, ηθ, γ]

In[*]:= P21γ[δ, α, σ, ωp, ηε, ηθ, γ]

In[*]:= P0γ[δ, α, σ, ωp, ηε, ηθ, γ]

```

## Fisher information

### generate

```

In[*]:= 
$$\frac{D[Pc\gamma[\delta, \alpha, \sigma, \omega p, \eta \epsilon, \eta \theta, \gamma], \delta]^2}{Pc\gamma[\delta, \alpha, \sigma, \omega p, \eta \epsilon, \eta \theta, \gamma]} +$$


$$\frac{D[P12\gamma[\delta, \alpha, \sigma, \omega p, \eta \epsilon, \eta \theta, \gamma], \delta]^2}{P12\gamma[\delta, \alpha, \sigma, \omega p, \eta \epsilon, \eta \theta, \gamma]} + \frac{D[P11\gamma[\delta, \alpha, \sigma, \omega p, \eta \epsilon, \eta \theta, \gamma], \delta]^2}{P11\gamma[\delta, \alpha, \sigma, \omega p, \eta \epsilon, \eta \theta, \gamma]} +$$


$$\frac{D[P22\gamma[\delta, \alpha, \sigma, \omega p, \eta \epsilon, \eta \theta, \gamma], \delta]^2}{P22\gamma[\delta, \alpha, \sigma, \omega p, \eta \epsilon, \eta \theta, \gamma]} + \frac{D[P21\gamma[\delta, \alpha, \sigma, \omega p, \eta \epsilon, \eta \theta, \gamma], \delta]^2}{P21\gamma[\delta, \alpha, \sigma, \omega p, \eta \epsilon, \eta \theta, \gamma]};$$


In[*]:= Simplify[%, TimeConstraint -> 1];

In[*]:= Fγ[δ_, α_, σ_, ωp_, ηε_, ηθ_, γ_] = %;

```

## output

```
In[*]:= F $\gamma$ [\delta, \alpha, \sigma, \omega\rho, \eta\epsilon, \eta\theta, \gamma]
```
